# Supplementary material for: Addressing intramolecular vibrational redistribution in a single molecule through pump and probe surface-enhanced vibrational spectroscopy
Source: arXiv:2601.02117 ancillary file (2026-05-04)
Supplement: Supplementary file 1 [file Supplementary_Information.pdf]

# Supporting Information for: Addressing intramolecular vibrational redistribution in a single molecule through pump and probe surface-enhanced vibrational spectroscopy

Aurelian Loirette-Pelous,<sup>1,2,3,\*</sup> Roberto A. Boto,<sup>2,4,5</sup> Javier Aizpurua,<sup>2,3,5</sup> and Ruben Esteban<sup>1,2,†</sup>

<sup>1</sup>*Centro de Física de Materiales CFM-MPC (CSIC-UPV/EHU),  
Paseo Manuel de Lardizabal 5, 20018 Donostia, Spain*

<sup>2</sup>*Donostia International Physics Center (DIPC),  
Paseo Manuel de Lardizabal 4, 20018 Donostia-San Sebastián, Spain*

<sup>3</sup>*Department of Electricity and Electronics, FCT-ZTF, UPV-EHU, Bilbao, 48080, Spain*

<sup>4</sup>*Department of Polymers and Advanced Materials, Faculty of Chemistry,  
The University of the Basque Country, UPV/EHU, Donostia 20018 Euskadi, Spain*

<sup>5</sup>*IKERBASQUE, Basque Foundation for Science, 48009 Bilbao, Spain*

## CONTENTS

|                                                                                           |    |
|-------------------------------------------------------------------------------------------|----|
| S1. Theoretical framework                                                                 | 2  |
| A. Molecular optomechanics description of SERS with independent vibrations                | 2  |
| B. Resonant laser pumping of a molecular vibration coupled to an infrared cavity          | 5  |
| C. Intramolecular vibrational redistribution via a Fermi resonance between two vibrations | 6  |
| S2. Pump-probe characterization of IVR                                                    | 8  |
| A. Signatures of IVR under continuous-wave Stokes SERS pumping                            | 8  |
| 1. Fermi resonance with $\omega_A = 2\omega_B$                                            | 8  |
| 2. Fermi resonance with $\omega_A \approx \omega_B + \omega_C$                            | 10 |
| B. Transient signatures of IVR under pulsed Stokes SERS pumping                           | 14 |
| 1. Fermi resonance with $\omega_A = 2\omega_B$                                            | 14 |
| 2. Fermi resonance with $\omega_A \approx \omega_B + \omega_C$                            | 15 |
| C. Signatures of IVR under continuous-wave infrared pumping                               | 17 |
| 1. Fermi resonance with $\omega_A = 2\omega_B$                                            | 17 |
| 2. Fermi resonance with $\omega_A \approx \omega_B + \omega_C$                            | 18 |
| S3. Discussion: additional considerations                                                 | 21 |
| S4. DFT calculations of the vibrational properties                                        | 23 |
| A. Details of the DFT calculations                                                        | 23 |
| B. Fermi resonances studied in this work                                                  | 24 |
| C. Effect of the gold atoms on the Fermi couplings for NBT                                | 24 |
| References                                                                                | 25 |

---

\* aurelianjoan.loirettepelous@ehu.eus

† ruben.esteban@ehu.eus

## S1. THEORETICAL FRAMEWORK

In Section II of the main text, we introduce the Hamiltonians and master equations describing the coupling of molecular vibrations between themselves and with optical and infrared (IR) cavities pumped with visible and infrared light. In this section, we describe in more detail the initial expressions and the derivation of the simplified equations.

### A. Molecular optomechanics description of SERS with independent vibrations

According to Eq. (1) and (2) of the main text, the Hamiltonian  $\hat{\mathcal{H}}_{\text{VIB}} + \hat{\mathcal{H}}_{\text{VIS}}(t)$  describing the optomechanical (Raman) interaction between the vibrational modes  $i$  of a single molecule and a single-mode optical cavity pumped by a laser can be written as [S1–S4]:

$$\hat{\mathcal{H}}_{\text{VIB}} + \hat{\mathcal{H}}_{\text{VIS}}(t) = \sum_i \hbar\omega_i \hat{b}_i^\dagger \hat{b}_i + \hbar\omega_{\text{VIS}}^{\text{cav}} \hat{a}_{\text{VIS}}^\dagger \hat{a}_{\text{VIS}} + i\hbar\Omega_{\text{VIS}}(t)(\hat{a}_{\text{VIS}}^\dagger e^{-i\omega_{\text{VIS}}t} - \hat{a}_{\text{VIS}} e^{i\omega_{\text{VIS}}t}) - \sum_i \hbar g_{\text{VIS},i} \hat{a}_{\text{VIS}}^\dagger \hat{a}_{\text{VIS}} (\hat{b}_i^\dagger + \hat{b}_i). \quad (\text{S1})$$

The first term in the right-hand side of Eq. (S1) describes the energy of the vibrations  $i$ , with  $\omega_i$  the vibrational frequency and  $\hat{b}_i^\dagger, \hat{b}_i$  the Bosonic vibration creation and annihilation operators. The second term describes the energy of the single-mode cavity, with  $\omega_{\text{VIS}}^{\text{cav}}$  the vibrational frequency and  $\hat{a}_{\text{VIS}}^\dagger, \hat{a}_{\text{VIS}}$  the Bosonic creation and annihilation operators of the cavity photons. The third term describes pumping of the optical cavity by a laser of frequency  $\omega_{\text{VIS}}$  in the visible range, with a pumping strength  $\Omega_{\text{VIS}}$ . It has been shown in Ref. [S5] that  $\Omega_{\text{VIS}}$  is related to the pumping intensity  $I_{\text{VIS}}$  by the relation:

$$\hbar\Omega_{\text{VIS}} = \frac{\hbar\kappa_{\text{VIS}}}{2} \sqrt{\frac{V_{\text{VIS}}}{\hbar\omega_{\text{VIS}}^{\text{cav}}}} K_{\text{VIS}} \sqrt{\frac{\sqrt{\varepsilon}}{c} I_{\text{VIS}}}, \quad (\text{S2})$$

where  $\kappa_{\text{VIS}}$  is the rate of incoherent photon losses from the cavity,  $V_{\text{VIS}}$  is the effective volume of the cavity quasi-normal mode (assumed to be single),  $K_{\text{VIS}}$  is the enhancement of the electric field of the laser at the position of the molecule,  $\varepsilon$  is the relative permittivity of the medium surrounding the plasmonic nanocavity and the molecule and  $c$  is the speed of light in vacuum. Finally, the fourth term in the right-hand side of Eq. (S1) describes the optomechanical interaction between the cavity and the vibrations. In particular, it has been shown in Refs. [S1, S6] that the optomechanical coupling strength is related to the Raman tensor  $\mathbf{R}_i$  of a vibration  $i$  by:

$$\hbar g_{\text{VIS},i} = \frac{\hbar\omega_{\text{VIS}}^{\text{cav}}}{2\sqrt{2}\hbar\omega_i} \frac{\hbar}{V_{\text{VIS}}} \frac{|\mathbf{e}_{\text{VIS}}^{\text{cav}} \cdot \mathbf{R}_i \cdot \mathbf{e}_{\text{VIS}}^{\text{cav}}|}{\varepsilon_0 \varepsilon} L_m^{1/4} |u_{\text{VIS}}^{\text{cav}}(\mathbf{r}_{\text{MOL}})|^2, \quad (\text{S3})$$

where the Raman tensor  $\mathbf{R}_i$  is the derivative of the molecule polarizability  $\boldsymbol{\alpha}$  with respect to the normal mode coordinate  $q_i$  of the vibration  $i$ , that is  $\mathbf{R}_i = [\partial\boldsymbol{\alpha}/\partial q_i](\mathbf{q} = \mathbf{0})$ ,  $\mathbf{e}_{\text{VIS}}^{\text{cav}}$  is the unit vector defining the polarization of the cavity mode,  $\varepsilon_0$  is the vacuum permittivity,  $L_m^{1/4} = (\varepsilon + 2)/3$  is a local field correction accounting for the difference between macroscopic and microscopic electric fields [S7],  $|u_{\text{VIS}}^{\text{cav}}(\mathbf{r})| \leq 1$  gives the spatial variation of the cavity mode electric field and  $\mathbf{r}_{\text{MOL}}$  indicates the position of the molecule. In this work, we assume that  $\varepsilon = L_m^{1/4} = 1$  and that the molecule is placed at the maximum field strength, so that  $|u_{\text{VIS}}^{\text{cav}}(\mathbf{r}_{\text{MOL}})| = 1$ . In addition, in ultrathin plasmonic nanogaps [S8], the cavity electric field is usually the largest in the direction perpendicular to the gap, that we note  $z$ . In this work, we thus only consider in Eq. (S3) the component  $R_i^{zz}$  of the Raman tensor of the molecule (see also Fig. S8).

We focus next on the interaction of the system composed of the cavity and the vibrations with its environment. The latter can be introduced by considering a Lindblad master equation that describes the temporal evolution of the density matrix  $\hat{\rho}$  of the molecule-cavity system [S2]:

$$\partial_t \hat{\rho} = \frac{i}{\hbar} [\hat{\rho}(t), \hat{\mathcal{H}}_{\text{VIB}} + \hat{\mathcal{H}}_{\text{VIS}}(t)] + \frac{\kappa_{\text{VIS}}}{2} (n_{\text{cav}}^{th} + 1) \mathcal{D}_{\hat{a}_{\text{VIS}}}[\hat{\rho}] + \frac{\kappa_{\text{VIS}}}{2} n_{\text{cav}}^{th} \mathcal{D}_{\hat{a}_{\text{VIS}}^\dagger}[\hat{\rho}] + \sum_i \frac{\gamma_i(1 + n_i^{th})}{2} \mathcal{D}_{\hat{b}_i}[\hat{\rho}] + \frac{\gamma_i n_i^{th}}{2} \mathcal{D}_{\hat{b}_i^\dagger}[\hat{\rho}], \quad (\text{S4})$$

where the Lindblad-Kossakowski terms are defined as  $\mathcal{D}_{\hat{O}}[\hat{\rho}] = 2\hat{O}\hat{\rho}\hat{O}^\dagger - \hat{O}^\dagger\hat{O}\hat{\rho} - \hat{\rho}\hat{O}^\dagger\hat{O}$ . The rates  $\gamma_i$  describe incoherent and non-radiative exchanges of vibrational excitations between a vibration  $i$  and a phonon bath in thermodynamic equilibrium at temperature  $T$ . The mean vibrational occupation is thus  $n_i^{th} = 1/[\exp(\hbar\omega_i/k_B T) - 1]$  when the vibration is thermalized with the bath. Similarly,  $\kappa_{\text{VIS}}$  describes the rate of incoherent exchange of photons between the cavity mode and a photon bath in thermodynamic equilibrium at temperature  $T$  with  $n_{\text{cav}}^{th} = 1/[\exp(\hbar\omega_{\text{VIS}}^{\text{cav}}/k_B T) - 1]$ . At

visible frequencies and for the temperatures considered in this work, the thermal occupation of the visible cavity is very low ( $n_{\text{cav}}^{th} \ll 1$ ) so that the terms  $\propto n_{\text{cav}}^{th}$  can be safely neglected in Eq. (S4). This yields Eq. (3) of the main text.

We then transform the cavity operators in the rotating frame of the laser, that is  $e^{i\omega_{\text{vis}}t}\hat{a}_{\text{vis}} \rightarrow \hat{a}_{\text{vis}}$  (resp.  $e^{-i\omega_{\text{vis}}t}\hat{a}_{\text{vis}}^\dagger \rightarrow \hat{a}_{\text{vis}}^\dagger$ ). We also introduce the (unitary) displacement operator  $\hat{U}(\alpha_{\text{vis}}) = e^{\alpha_{\text{vis}}\hat{a}_{\text{vis}}^\dagger - \alpha_{\text{vis}}^*\hat{a}_{\text{vis}}}$  that shifts the cavity creation operators by the coherent amplitude  $\alpha_{\text{vis}}$ , so that  $\hat{U}^\dagger(\alpha_{\text{vis}})\hat{a}_{\text{vis}}\hat{U}(\alpha_{\text{vis}}) = \alpha_{\text{vis}} + \hat{a}_{\text{vis}}$ . Under continuous-wave excitation, a convenient parametrization for  $\alpha_{\text{vis}}$  is:

$$\alpha_{\text{vis}} = \frac{-i\Omega_{\text{vis}}}{\omega_{\text{vis}}^{\text{cav}} - \omega_{\text{vis}} - i\kappa_{\text{vis}}/2}. \quad (\text{S5})$$

For pulsed excitation, the unitary transformation  $\hat{U}(\alpha_{\text{vis}})$  introduces in principle a term proportional to the time derivative of  $\hat{U}(\alpha_{\text{vis}})$  in the Hamiltonian. However, if the temporal variations of the pumping envelope  $\Omega_{\text{vis}}(t)$  are slow relative to the cavity photon residence time (as in our work, see further discussion in Section S2 B),  $\alpha_{\text{vis}}(t)$  evolves adiabatically in response to  $\Omega_{\text{vis}}(t)$ , so that the derivative of  $\hat{U}(\alpha_{\text{vis}})$  is neglected when applying the transformation with the parametrization given in Eq. (S5).

According to these transformations, the Hamiltonian  $\hat{\mathcal{H}}_{\text{vib}} + \hat{\mathcal{H}}_{\text{vis}}(t)$  is replaced by:

$$\begin{aligned} \hat{\mathcal{H}}_{\text{vib}} + \hat{\mathcal{H}}_{\text{vis}}^{\alpha_{\text{vis}}}(t) = & \sum_i \hbar\omega_i \hat{b}_i^\dagger \hat{b}_i + \hbar(\omega_{\text{vis}}^{\text{cav}} - \omega_{\text{vis}})\hat{a}_{\text{vis}}^\dagger \hat{a}_{\text{vis}} \\ & - \sum_i \hbar g_{\text{vis},i} |\alpha_{\text{vis}}(t)| (\hat{a}_{\text{vis}}^\dagger + \hat{a}_{\text{vis}})(\hat{b}_i^\dagger + \hat{b}_i) - \sum_i \hbar g_{\text{vis},i} \hat{a}_{\text{vis}}^\dagger \hat{a}_{\text{vis}} (\hat{b}_i^\dagger + \hat{b}_i), \end{aligned} \quad (\text{S6})$$

where we have also applied a transformation  $\hat{a}_{\text{vis}} \rightarrow e^{i\arg[\alpha_{\text{vis}}]}\hat{a}_{\text{vis}}$ , with  $\arg[\alpha_{\text{vis}}]$  the argument of  $\alpha_{\text{vis}}$ , so that  $\alpha_{\text{vis}}^* \hat{a}_{\text{vis}} + \alpha_{\text{vis}} \hat{a}_{\text{vis}}^\dagger$  can be replaced by  $|\alpha_{\text{vis}}|(\hat{a}_{\text{vis}} + \hat{a}_{\text{vis}}^\dagger)$ . We have neglected in Eq. (S6) and in the following sections a term  $\hbar g_{\text{vis},i} |\alpha_{\text{vis}}(t)|^2 (\hat{b}_i^\dagger + \hat{b}_i)$ , which gives a coherent displacement of the vibration operator, because its effect in the SERS spectra and phonon populations can be neglected in typical conditions [S9]. We further emphasize that the transformations that have been introduced leave the Lindbladians unchanged in the master equation. The Hamiltonian Eq. (S6) is equivalent to Eq. (S1) and serves as a convenient starting point to introduce two main approximations that greatly simplify the resolution of the master equation of the system. The first approximation consists in neglecting the terms  $\hbar g_{\text{vis},i} \hat{a}_{\text{vis}}^\dagger \hat{a}_{\text{vis}} (\hat{b}_i^\dagger + \hat{b}_i)$  in Eq. (S6), which is known as the *linearization approximation*. This approximation is justified when the optomechanical system operates in the weak coupling regime  $g_{\text{vis},i} \ll \kappa_{\text{vis}}$  [S2], as it is by far the case for the parameters considered in this work (see Section III.A of the main text). The second approximation is based on the different time scales for the exchanges between the cavity and its environment, and for the vibrations and their environment, respectively. Indeed, the rates  $\hbar\gamma_i$  associated to the vibrations are typically in the  $\sim 1$  meV range, while the rate  $\hbar\kappa_{\text{vis}}$  associated to the visible cavity is in the  $\sim 100$  meV range, so that relaxation after a perturbation is  $\sim 100$  times faster for the cavity compared to the vibrations. Hence, from the point of view of the vibrations, the cavity degrees of freedom are always in a steady-state, that is, evolve adiabatically under variations of the vibrational degrees of freedom. In addition, the vibrations and the cavity are always weakly coupled ( $g_{\text{vis},i} \ll \kappa_{\text{vis}}$ ) for the parameters used in this work (see Section III A of the main text), so that there is no reversible exchanges between the vibrations and the cavity. Therefore, the second approximation that we implement is the so-called *adiabatic approximation* (also called Markovian approximation) that consists in eliminating the cavity degrees of freedom, which yields a new master equation for the reduced density matrix of the vibrational degrees of freedom only [S10–S12]. According to Refs. [S9, S12, S13], the master equation for the reduced density matrix  $\hat{\rho}_{\text{vib}}$  can be written as:

$$\partial_t \hat{\rho}_{\text{vib}} = \frac{i}{\hbar} [\hat{\rho}_{\text{vib}}, \sum_i \hbar(\omega_i + \Delta_i) \hat{b}_i^\dagger \hat{b}_i] + \sum_i \frac{1}{2} [\gamma_i(1 + n_i^{th}) + \Gamma_i^-] \mathcal{D}_{\hat{b}_i} [\hat{\rho}_{\text{vib}}] + \sum_i \frac{1}{2} [\gamma_i n_i^{th} + \Gamma_i^+] \mathcal{D}_{\hat{b}_i^\dagger} [\hat{\rho}_{\text{vib}}], \quad (\text{S7})$$

where:

$$\Gamma_i^\pm = \frac{|\alpha_{\text{vis}}|^2 g_{\text{vis},i}^2 \kappa_{\text{vis}}}{(\omega_{\text{vis}} \mp \omega_i - \omega_{\text{vis}}^{\text{cav}})^2 + (\kappa_{\text{vis}}/2)^2} = \frac{V_{\text{vis}} K_{\text{vis}}^2}{c \hbar \omega_{\text{vis}}^{\text{cav}}} \times \frac{1}{4 \left( \frac{\omega_{\text{vis}} - \omega_{\text{vis}}^{\text{cav}}}{\kappa} \right)^2 + 1} \times \frac{g_{\text{vis},i}^2 \kappa_{\text{vis}}}{(\omega_{\text{vis}} \mp \omega_i - \omega_{\text{vis}}^{\text{cav}})^2 + (\kappa_{\text{vis}}/2)^2} \times I_{\text{vis}}, \quad (\text{S8})$$

and:

$$\Delta_i = - \left[ \Gamma_i^+ \frac{\omega_{\text{vis}}^{\text{cav}} - \omega_{\text{vis}} + \omega_i}{\kappa_{\text{vis}}} + \Gamma_i^- \frac{\omega_{\text{vis}}^{\text{cav}} - \omega_{\text{vis}} - \omega_i}{\kappa_{\text{vis}}} \right]. \quad (\text{S9})$$

In Eq. (S7), the terms  $\Gamma_i^-$  are rates of incoherent vibrational relaxation while the terms  $\Gamma_i^+$  are rates of incoherent vibrational excitation. In particular,  $\Gamma_i^+$  involves a resonance at  $(\omega_{\text{vis}} - \omega_i - \omega_{\text{vis}}^{\text{cav}})^2$ , which indicates that a Stokes process is involved (the resonance of  $\Gamma_i^+$  occurs when the Stokes photon at frequency  $\omega_i + \omega_{\text{vis}}^{\text{cav}}$  is resonant with the cavity). Similarly,  $\Gamma_i^-$  involves a resonance at  $(\omega_{\text{vis}} + \omega_i - \omega_{\text{vis}}^{\text{cav}})^2$  indicating an anti-Stokes process. The terms  $\Delta_i$  are called spring shifts [S14] and account for a shift of the vibrational frequency that is proportional to the pumping intensity. The  $\Delta_i$  are expected to be negligible for a single molecule in a plasmonic nanocavity with the pumping intensities considered in this work (see e.g. Eq. (5) of Ref. [S15]), and therefore we omit these terms from here on. We also note that in the adiabatic approximation, the coupling of several vibrations to a common cavity yields intervibrational coupling terms  $\propto \mathcal{D}_{\hat{b}_i^\dagger \hat{b}_j}[\hat{\rho}_{\text{vib}}]$ ,  $\mathcal{D}_{\hat{b}_i \hat{b}_j^\dagger}[\hat{\rho}_{\text{vib}}]$  [S9]. However, we only consider in this work vibrations with large detunings  $|\omega_i - \omega_j| \gg \gamma_i, \gamma_j$ , so that these terms are strongly non-resonant and thus negligible.

We now focus on the population  $n_i(t) \equiv \langle \hat{b}_i^\dagger \hat{b}_i \rangle(t) \equiv \text{Tr}[\hat{b}_i^\dagger \hat{b}_i \hat{\rho}_{\text{vib}}(t)]$  of a vibration  $i$ . Starting from Eq. (S7), it is straightforward to derive the equation ruling the dynamics of  $n_i(t)$ :

$$\partial_t n_i = -(\gamma_i + \Gamma_i^-)n_i + \Gamma_i^+(n_i + 1) + \gamma_i n_i^{\text{th}}. \quad (\text{S10})$$

Under continuous-wave (or slow-envelope) illumination, Eq. (S10) then yields the steady state  $n_i = n_i^{\text{th}} + \Gamma_i^+ / [\gamma_i + \Gamma_i^- - \Gamma_i^+]$ . Finally, we focus in this work on low-to-moderate pumping intensities so that  $\gamma_i \gg |\Gamma_i^- - \Gamma_i^+|$  [S3]. This yields  $n_i = n_i^{\text{th}} + \Gamma_i^+ / \gamma_i$ , which is the relation reported in Eq. (4) of the main text.

Lastly, we focus on SERS spectra. Under continuous-wave or slow-envelope illumination, SERS spectra in the reference frame of the incident laser are derived from the general expression [S16]:

$$I(\omega, t) \propto \omega^4 \kappa_{\text{vis}} \text{Re} \int_0^\infty d\tau e^{-i(\omega - \omega_{\text{vis}})\tau} \langle \hat{a}_{\text{vis}}^\dagger(t + \tau) \hat{a}_{\text{vis}}(t) \rangle, \quad (\text{S11})$$

where  $t$  accounts for the time evolution of  $\Omega_{\text{vis}}(t)$  (that must be slow relative to the oscillation frequency  $\omega_{\text{vis}}$  of the incident field) and  $\omega^4$  accounts for the frequency-dependence of dipolar emission. In the linearization and adiabatic approximations, Eq. (S11) can be conveniently expressed in term of the vibrational operators instead of the photon operators. In particular, it was shown in Ref. [S9, S13] that the Stokes and anti-Stokes SERS spectra of a single-mode cavity can be cast into the respective forms:

$$I^S(\omega, t) \propto \omega^4 \sum_i \Gamma_i^+ \text{Re} \int_0^\infty d\tau e^{-i(\omega - \omega_{\text{vis}})\tau} \langle \hat{b}_i(t + \tau) \hat{b}_i^\dagger(t) \rangle, \quad (\text{S12})$$

and

$$I^{aS}(\omega, t) \propto \omega^4 \sum_i \Gamma_i^- \text{Re} \int_0^\infty d\tau e^{-i(\omega - \omega_{\text{vis}})\tau} \langle \hat{b}_i^\dagger(t + \tau) \hat{b}_i(t) \rangle. \quad (\text{S13})$$

Next, Eqs. (S12), (S13) can be simplified using the quantum regression theorem [S17], which states that the evolution of the correlation  $\langle \hat{b}_i^\dagger(t + \tau) \hat{b}_i(t) \rangle$  with time  $\tau \geq 0$  is the same as the dynamical evolution of the coherence  $\langle \hat{b}_i^\dagger(\tau) \rangle$  but with initial condition  $\langle \hat{b}_i^\dagger(t) \hat{b}_i(t) \rangle = n_i(t)$  (and similarly for  $\langle \hat{b}_i(t + \tau) \hat{b}_i^\dagger(t) \rangle$  with  $\langle \hat{b}_i(\tau) \rangle$  and  $\langle \hat{b}_i(t) \hat{b}_i^\dagger(t) \rangle = 1 + n_i(t)$ ). According to the master equation Eq. (S7), the dynamics of  $\langle \hat{b}_i^\dagger(\tau) \rangle$  reads:

$$\partial_\tau \langle \hat{b}_i^\dagger(\tau) \rangle = [i\omega_i + \frac{\gamma_i + \Gamma_i^-(t) - \Gamma_i^+(t)}{2}] \langle \hat{b}_i^\dagger(\tau) \rangle, \quad (\text{S14})$$

so that  $\langle \hat{b}_i^\dagger(t + \tau) \hat{b}_i(t) \rangle = n_i(t) e^{i\omega_i \tau} e^{-[\gamma_i + \Gamma_i^-(t) - \Gamma_i^+(t)]\tau/2}$  and  $\langle \hat{b}_i(t + \tau) \hat{b}_i^\dagger(t) \rangle = [1 + n_i(t)] e^{-i\omega_i \tau} e^{-[\gamma_i + \Gamma_i^-(t) - \Gamma_i^+(t)]\tau/2}$ . Inserting the later results in Eqs. (S12), (S13) then yields:

$$I^S(\omega, t) \propto \omega^4 \sum_i \Gamma_i^+ \frac{(\gamma_i + \Gamma_i^-(t) - \Gamma_i^+(t))/2}{(\omega - \omega_{\text{vis}} + \omega_i)^2 + (\gamma_i + \Gamma_i^-(t) - \Gamma_i^+(t))^2/4} n_i(t). \quad (\text{S15})$$

and

$$I^{aS}(\omega, t) \propto \omega^4 \sum_i \Gamma_i^- \frac{(\gamma_i + \Gamma_i^-(t) - \Gamma_i^+(t))/2}{(\omega - \omega_{\text{vis}} - \omega_i)^2 + (\gamma_i + \Gamma_i^-(t) - \Gamma_i^+(t))^2/4} [1 + n_i(t)]. \quad (\text{S16})$$

For continuous-wave (or slow-envelope) illumination and focusing on a single vibration  $i$ , frequency integration of Eq. (S16) yields Eq. (5) reported in the main text.

## B. Resonant laser pumping of a molecular vibration coupled to an infrared cavity

In this section, we focus on the coupling of molecular vibrations to an IR cavity illuminated by IR light. Although similar to the scenario discussed in the previous section, we note that this case involves a distinct type of coupling term that must be addressed.

According to Eq. (1) and (6) of the main text, the Hamiltonian describing the dipolar interaction between a single vibration  $i$  in a single molecule and a single-mode of an infrared cavity pumped by an infrared laser of frequency  $\omega_{\text{IR}}$  can be written as [S18, S19]:

$$\hat{\mathcal{H}}_{\text{VIB},i} + \hat{\mathcal{H}}_{\text{IR},i}(t) = \hbar\omega_i \hat{b}_i^\dagger \hat{b}_i + \hbar\omega_{\text{IR}}^{\text{cav}} \hat{a}_{\text{IR}}^\dagger \hat{a}_{\text{IR}} + i\hbar\Omega_{\text{IR}}(t)(\hat{a}_{\text{IR}}^\dagger e^{-i\omega_{\text{IR}}t} - \hat{a}_{\text{IR}} e^{i\omega_{\text{IR}}t}) - \hbar g_{\text{IR},i}(\hat{a}_{\text{IR}}^\dagger \hat{b}_i + \hat{a}_{\text{IR}} \hat{b}_i^\dagger). \quad (\text{S17})$$

The first and second terms in the right-hand side of Eq. (S17) describes the energy of the vibration  $i$  and of the single-mode infrared cavity, respectively. The third term describes pumping of the IR cavity by an IR laser of frequency  $\omega_{\text{IR}}$ , with a pumping strength  $\Omega_{\text{IR}}$ . As for visible pumping (see Eq. (S2)),  $\Omega_{\text{IR}}$  is related to the pumping intensity  $I_{\text{IR}}$  by the relation:

$$\hbar\Omega_{\text{IR}} = \frac{\hbar\kappa_{\text{IR}}}{2} \sqrt{\frac{V_{\text{IR}}}{\hbar\omega_{\text{IR}}^{\text{cav}}}} K_{\text{IR}} \sqrt{\frac{\sqrt{\epsilon} I_{\text{IR}}}{c}}. \quad (\text{S18})$$

Finally, the fourth term in the right-hand side of Eq. (S17) describes the dipolar interaction between the IR cavity and the vibrations, with coupling strength:

$$\hbar g_{\text{IR},i} = \sqrt{\frac{\hbar\omega_i}{2V_{\text{IR}}\epsilon_0\epsilon}} \mathbf{d}_i \cdot \mathbf{e}_{\text{IR}}^{\text{cav}} |u_{\text{IR}}^{\text{cav}}(\mathbf{r})|^2, \quad (\text{S19})$$

where  $\mathbf{d}_i$  is the derivative of the molecule dipole moment  $\boldsymbol{\mu}$  with respect to the coordinate  $q_i$  of the mode  $i$  [S20], that is  $\mathbf{d}_i \equiv [\partial\boldsymbol{\mu}/\partial q_i](\mathbf{q} = \mathbf{0})$ ,  $\mathbf{e}_{\text{IR}}^{\text{cav}}$  is the unit vector defining the polarization of the IR cavity mode,  $|u_{\text{IR}}^{\text{cav}}(\mathbf{r})| \leq 1$  gives the spatial variation of the electric field of the mode and  $\mathbf{r}_{\text{MOL}}$  indicates the position of the molecule. In this work, we assume that the molecule is placed at the maximum field strength, so that  $|u_{\text{IR}}^{\text{cav}}(\mathbf{r}_{\text{MOL}})| = 1$ . In addition, we assume that the electric field of the IR cavity is the largest in the direction perpendicular to the gap (noted  $z$ ), so that we only consider the component  $d_i^z = \mathbf{d}_i \cdot \mathbf{e}_z$  of the dipole moment of the vibrations.

In this case, the Lindblad master equation for the density matrix  $\hat{\rho}$  of the molecule-cavity system is [S2]:

$$\partial_t \hat{\rho} = \frac{i}{\hbar} [\hat{\rho}(t), \hat{\mathcal{H}}_{\text{VIB},i} + \hat{\mathcal{H}}_{\text{IR},i}(t)] + \frac{\kappa_{\text{IR}}}{2} (n_{\text{cav}}^{th} + 1) \mathcal{D}_{\hat{a}_{\text{IR}}}[\hat{\rho}] + \frac{\kappa_{\text{IR}}}{2} n_{\text{cav}}^{th} \mathcal{D}_{\hat{a}_{\text{IR}}^\dagger}[\hat{\rho}] + \frac{\gamma_i(1 + n_i^{th})}{2} \mathcal{D}_{\hat{b}_i}[\hat{\rho}] + \frac{\gamma_i n_i^{th}}{2} \mathcal{D}_{\hat{b}_i^\dagger}[\hat{\rho}], \quad (\text{S20})$$

where the term  $\propto \gamma_i n_i^{th}$  is kept, differently to Eq. (S4), as thermal occupations at IR frequencies and cryogenic temperatures may be close to 1.

We then introduce again (Section S1 A) the rotating frame of the IR laser, that we also apply to the vibration (i.e.  $e^{i\omega_{\text{IR}}t} \hat{a}_{\text{IR}} \rightarrow \hat{a}_{\text{IR}}$  and  $e^{i\omega_{\text{IR}}t} \hat{b}_i \rightarrow \hat{b}_i$ ), and the displacement operator  $\hat{U}(\alpha_{\text{IR}}) = e^{\alpha_{\text{IR}} \hat{a}_{\text{IR}}^\dagger - \alpha_{\text{IR}}^* \hat{a}_{\text{IR}}}$  with:

$$\alpha_{\text{IR}}(t) = \frac{\Omega_{\text{IR}}(t)}{i(\omega_{\text{IR}}^{\text{cav}} - \omega_{\text{IR}}) + \kappa_{\text{IR}}/2}, \quad (\text{S21})$$

so that the Hamiltonian  $\hat{\mathcal{H}}_{\text{VIB},i} + \hat{\mathcal{H}}_{\text{IR},i}(t)$  transforms in:

$$\hat{\mathcal{H}}_{\text{VIB},i} + \hat{\mathcal{H}}_{\text{IR},i}^{\alpha_{\text{IR}}} = \hbar(\omega_i - \omega_{\text{IR}}) \hat{b}_i^\dagger \hat{b}_i + \hbar(\omega_{\text{IR}}^{\text{cav}} - \omega_{\text{IR}}) \hat{a}_{\text{IR}}^\dagger \hat{a}_{\text{IR}} - \hbar g_{\text{IR},i} |\alpha_{\text{IR}}| (\hat{b}_i + \hat{b}_i^\dagger) - \hbar g_{\text{IR},i} (\hat{a}_{\text{IR}}^\dagger \hat{b}_i + \hat{a}_{\text{IR}} \hat{b}_i^\dagger), \quad (\text{S22})$$

while the Lindbladians  $\mathcal{D}_{\hat{a}_{\text{IR}}^\dagger}[\hat{\rho}]$ ,  $\mathcal{D}_{\hat{a}_{\text{IR}}}[\hat{\rho}]$ ,  $\mathcal{D}_{\hat{b}_i^\dagger}[\hat{\rho}]$  and  $\mathcal{D}_{\hat{b}_i}[\hat{\rho}]$  into Eq. (S20) are left unchanged.

Next, we note that the rate  $\hbar\kappa_{\text{IR}}$  associated to the IR cavity losses typically lies in the  $\gtrsim 10$  meV range [S21, S22] while the vibrational decay rate typically lies in the  $\hbar\gamma_i \sim 1$  meV range, so that the inequality  $\hbar\kappa_{\text{IR}} \gg \hbar\gamma_i$  is satisfied. In addition, in this work the IR cavity and the molecule are always weakly coupled ( $g_{\text{IR},i} \ll \kappa_{\text{IR}}$ , see parameters used in Section III A of the main text). Hence, we can apply the adiabatic approximation, so that the master equation (S20) can be transformed into the following master equation of the reduced density matrix  $\hat{\rho}_{\text{VIB}}$ :

$$\partial_t \hat{\rho}_{\text{VIB}} = \frac{i}{\hbar} [\hat{\rho}_{\text{VIB}}, \hbar(\omega_i - \omega_{\text{IR}} + \Delta_{\text{IR},i}) \hat{b}_i^\dagger \hat{b}_i - \hbar g_{\text{IR},i} (\alpha_{\text{IR}}^* \hat{b}_i + \alpha_{\text{IR}} \hat{b}_i^\dagger)] + \frac{1}{2} \gamma_i' (1 + n_i^{th}) \mathcal{D}_{\hat{b}_i}[\hat{\rho}_{\text{VIB}}] + \frac{1}{2} \gamma_i' n_i^{th} \mathcal{D}_{\hat{b}_i^\dagger}[\hat{\rho}_{\text{VIB}}], \quad (\text{S23})$$

where:

$$\gamma'_i = \gamma_i + \frac{g_{\text{IR},i}^2 \kappa_{\text{IR}}}{(\omega_{\text{IR}}^{\text{cav}} - \omega_i)^2 + (\kappa_{\text{IR}}/2)^2} \text{ and } \Delta_{\text{IR},i} = (\gamma'_i - \gamma_i) \frac{\omega_{\text{IR}}^{\text{cav}} - \omega_i}{\kappa_{\text{IR}}}. \quad (\text{S24})$$

Considering the typical values of  $g_{\text{IR},i}$ ,  $\kappa_{\text{IR}}$  and  $\gamma_i$  given in Section III.A of the main text, we can approximate  $\gamma'_i \approx \gamma_i$  and  $\Delta_{\text{IR},i} \approx 0$  in Eq. (S23). Accordingly, the population  $n_i(t) \equiv \langle \hat{b}_i^\dagger \hat{b}_i \rangle$  of a vibration  $i$  can be determined by solving the set of equations:

$$\partial_t n_i = -\gamma_i (n_i - n_i^{\text{th}}) + 2g_{\text{IR},i} \text{Im}[\alpha_{\text{IR}}^*(t) \langle \hat{b}_i \rangle], \quad (\text{S25})$$

and

$$\partial_t \langle \hat{b}_i \rangle = -[i(\omega_i - \omega_{\text{IR}}) + \frac{\gamma_i}{2}] \langle \hat{b}_i \rangle + ig_{\text{IR},i} \alpha_{\text{IR}}(t), \quad (\text{S26})$$

where  $\langle \hat{b}_i \rangle$  is the coherent amplitude of vibration  $i$ . Under continuous-wave (or slow-envelope) illumination, the set of equations can be solved analytically and yields:

$$n_i^{\text{cw}} = n_i^{\text{th}} + \frac{g_{\text{IR},i}^2 |\alpha_{\text{IR}}|^2}{(\omega_i - \omega_{\text{IR}})^2 + (\gamma_i/2)^2} = n_i^{\text{th}} + |\langle \hat{b}_i \rangle|^2. \quad (\text{S27})$$

which corresponds to equation (7) in the main text.

### C. Intramolecular vibrational redistribution via a Fermi resonance between two vibrations

In this section, we provide a complementary discussion to the results presented in Section II.B.2 of the main text, by analyzing in more detail the effects of a Fermi resonance between two vibrations in the weak and strong coupling regimes. To focus on the effect of the Fermi resonance, we do not include here the excitation by light or the coupling with a cavity.

We start from the total Hamiltonian describing the coupling of the fundamental of a vibration A and the overtone of a vibration B by a Fermi resonance is obtained by combining Eq. (1) and Eq. (9) of the main text:

$$\hat{\mathcal{H}}_{\text{VIB},A} + \hat{\mathcal{H}}_{\text{VIB},B} + \hat{\mathcal{H}}_F = \hbar\omega_A \hat{b}_A^\dagger \hat{b}_A + \hbar\omega_B \hat{b}_B^\dagger \hat{b}_B + \hbar g_F (\hat{b}_A (\hat{b}_B^\dagger)^2 + \hat{b}_A^\dagger \hat{b}_B^2), \quad (\text{S28})$$

where  $g_F$  is the coupling strength of the Fermi resonance. The first and second terms in the right-hand side of Eq. (S28) describes the energy of vibrations A and B, respectively, and the third term account for the Fermi resonance coupling.

We focus first on the case in which the coupling strength  $g_F$  in the Hamiltonian Eq. (S28) is small with respect to the vibrational modes decay rates, that is  $2\sqrt{2}g_F \lesssim \gamma_A + \gamma_B$  (weak coupling [S23]). In this case, a description of the system in term of the bare vibrational operators  $\hat{b}_A$  and  $\hat{b}_B$  is advantageous [S24]. Accordingly, the master equation ruling the evolution of the matrix density  $\hat{\rho}_{\text{VIB}}$  of the vibrational system can be directly analyzed in the form:

$$\partial_t \hat{\rho}_{\text{VIB}} = \frac{i}{\hbar} [\hat{\rho}(t), \hat{\mathcal{H}}_{\text{VIB},A} + \hat{\mathcal{H}}_{\text{VIB},B} + \hat{\mathcal{H}}_F] + \sum_{i=A,B} \frac{\gamma_i(1 + n_i^{\text{th}})}{2} \mathcal{D}_{\hat{b}_i}[\hat{\rho}_{\text{VIB}}] + \frac{\gamma_i n_i^{\text{th}}}{2} \mathcal{D}_{\hat{b}_i^\dagger}[\hat{\rho}_{\text{VIB}}]. \quad (\text{S29})$$

It is then insightful to look for the vibrational populations in the presence of the Fermi resonance. According to Eq. (S29), the populations of vibrations A and B follow the set of equations:

$$\frac{dn_A}{dt} = -\gamma_A (n_A - n_A^{\text{th}}) + 2g_F \text{Im}[\langle \hat{b}_B^2 \hat{b}_A^\dagger \rangle], \quad (\text{S30})$$

$$\frac{dn_B}{dt} = \gamma_B (n_B - n_B^{\text{th}}) - 4g_F \text{Im}[\langle \hat{b}_B^2 \hat{b}_A^\dagger \rangle], \quad (\text{S31})$$

$$\frac{d\langle \hat{b}_B^2 \hat{b}_A^\dagger \rangle}{dt} = - \left[ -i(\omega_A - 2\omega_B) + \frac{(\gamma_A + 2\gamma_B)}{2} \right] \langle \hat{b}_B^2 \hat{b}_A^\dagger \rangle - ig_F (4\langle \hat{n}_B \hat{n}_A \rangle + 2n_A + n_B - \langle \hat{n}_B^2 \rangle), \quad (\text{S32})$$

which shows that the population transfer between vibration A and vibration B is mediated by the correlation  $\langle \hat{b}_B^2 \hat{b}_A^\dagger \rangle$ . In particular, in the steady-state the above equations simplify to:

$$n_A = n_A^{th} - \frac{4g_{F,\text{eff}}^2}{\gamma_A(\gamma_A + 2\gamma_B)}(4\langle \hat{n}_B \hat{n}_A \rangle + 2n_A + n_B - \langle \hat{n}_B^2 \rangle), \quad (\text{S33})$$

$$n_B = n_B^{th} + \frac{8g_{F,\text{eff}}^2}{\gamma_A(\gamma_A + 2\gamma_B)}(4\langle \hat{n}_B \hat{n}_A \rangle + 2n_A + n_B - \langle \hat{n}_B^2 \rangle), \quad (\text{S34})$$

where we introduce the shorthand:

$$g_{F,\text{eff}} = \frac{g_F}{\sqrt{1 + 4\left(\frac{\omega_A - 2\omega_B}{\gamma_A + 2\gamma_B}\right)^2}}. \quad (\text{S35})$$

The quantity  $g_{F,\text{eff}}$  can be interpreted as an effective Fermi resonance coupling strength that accounts for the detuning between the fundamental of vibration A and the overtone of vibration B. The effect of the detuning is to reduce the effective coupling strength of the Fermi resonance, and this reduction depends on the intrinsic loss rate of the vibrations involved in the Fermi resonance. In particular, a Fermi resonance is efficient as long as the detuning between the fundamental vibration A and the overtone of vibration B remains small or comparable to the vibrational decay rate. Finally, we note that in the present case of weak coupling between the vibrations, the anti-Stokes SERS spectra exhibits the same overall shape as for independent vibrations, with a single emission peak associated to each vibrational mode, but with peak amplitudes (see Eq. (5) of the main text) that are affected by the Fermi resonance through its influence on the vibrational populations (Eqs. (S33), (S34)). The width of the peaks is also enhanced, as a Fermi resonance is a new decay channel, but this enhancement does not depend on vibrational populations.

We consider next the strong coupling regime ( $2\sqrt{2}g_F > \gamma_A + \gamma_B$ ). In addition, we restrict here our study to the following subset of states:  $|1, 0\rangle$ , corresponding to the fundamental of vibration A;  $|0, 2\rangle$ , corresponding to the overtone of vibration B; and  $|0, 1\rangle$ , corresponding to the fundamental of vibration B. In this basis, the Hamiltonian Eq. (S28) reads:

$$\hat{\mathcal{H}}_{\text{VIB},A} + \hat{\mathcal{H}}_{\text{VIB},B} + \hat{\mathcal{H}}_F = \hbar\omega_A|1, 0\rangle\langle 1, 0| + \hbar\omega_B|0, 1\rangle\langle 0, 1| + 2\hbar\omega_B|0, 2\rangle\langle 0, 2| + \sqrt{2}\hbar g_F(|0, 2\rangle\langle 1, 0| + |1, 0\rangle\langle 0, 2|). \quad (\text{S36})$$

In this form, the Hamiltonian (S36) can be straightforwardly diagonalized into:

$$\hat{\mathcal{H}}_{\text{VIB},A} + \hat{\mathcal{H}}_{\text{VIB},B} + \hat{\mathcal{H}}_F = \hbar\omega_U|U\rangle\langle U| + \hbar\omega_L|L\rangle\langle L| + \hbar\omega_B|0, 1\rangle\langle 0, 1|, \quad (\text{S37})$$

where the mixed eigenstates  $|U\rangle$  and  $|L\rangle$  are defined as [S16]:

$$|U\rangle = C|1, 0\rangle + X|0, 2\rangle \quad \text{and} \quad |L\rangle = X|1, 0\rangle - C|0, 2\rangle, \quad (\text{S38})$$

with  $C = (1/\sqrt{2})\sqrt{1 + (\omega_A - 2\omega_B)/2\Delta}$ ,  $X = (1/\sqrt{2})\sqrt{1 - (\omega_A - 2\omega_B)/4\Delta}$ ,  $\Delta = \sqrt{2g_F^2 + (\omega_A - 2\omega_B)^2/4}$ , and with frequencies  $\omega_U = (\omega_A + 2\omega_B)/2 + \sqrt{(\omega_A - 2\omega_B)^2/4 + 2g_F^2}$ ,  $\omega_L = (\omega_A + 2\omega_B)/2 - \sqrt{(\omega_A - 2\omega_B)^2/4 + 2g_F^2}$ .

In summary, when the vibrations are strongly coupled, the Hamiltonian (S37) defines the new eigenstates of the system, that are the states that can be observed through Raman or infrared spectroscopy. In particular, here the Fermi resonance coupling leads to the hybridization of the fundamental of vibration A and of the overtone of vibration B into an upper and a lower mixed state. On the other hand, the fundamental of vibration B remains unchanged. For a perfectly resonant Fermi resonance ( $\omega_A = 2\omega_B$ ), the states  $|U\rangle$ ,  $|L\rangle$  given in Eq. (S38) as well as their energies reduce to those given in Section II.B.2 and in Figure 1. (b) of the main text. In addition, all this analysis can be readily generalized to the case of a Fermi resonance involving 3 vibrations as studied in Sections S2.A.2, S2.B.2 and S2.C.2.

In conclusion, a system in the strong coupling regime exhibits qualitative differences compared to a system in the weak coupling regime, as we have shown by writing the Hamiltonian of the former in terms of the mixed states (Eqs. (S38)). In particular, the strong coupling point of view of the vibrational states is insightful for analyzing the presence of a Fermi doublet at frequencies  $\sim \omega_A$  in the SERS spectra, as seen in Fig. 2 (b), 3 (c) and 5 (c) of the main text. However, we emphasize that the Hamiltonian and master equation in term of the uncoupled basis (Eqs. (S28) and (S29)) can be generally applied to obtain the numerical solution [S25], which is the approach that we follow to obtain all results.

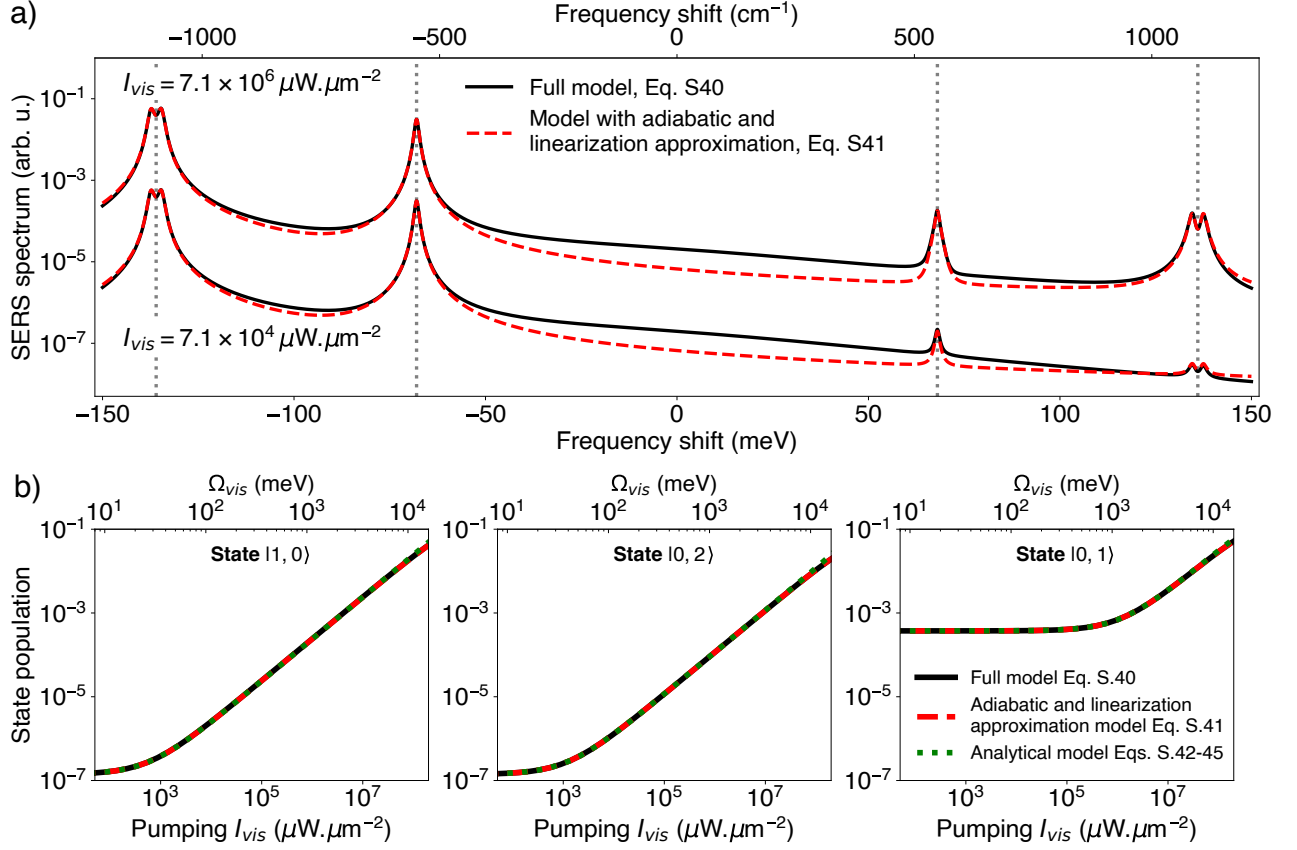

FIG. S1. Comparison of models used to analyze the importance of IVR under cw Stokes SERS pumping and cw anti-Stokes SERS probing. The configuration under study is sketched in Fig. 3 (a) of the main text. Black continuous lines show results obtained by solving the full master equation (S40). Red dashed lines are computed by solving the master equation (S41), obtained using linearization and adiabatic elimination of the cavity degrees of freedom. The Green dotted lines on panel (b) correspond to solutions of the set of approximated equations (S42-S45). (a): anti-Stokes SERS spectra of two molecular vibrations coupled by the Fermi resonance, for two pumping intensities  $I_{vis} = 7.1 \times 10^4 \mu\text{W} \cdot \mu\text{m}^{-2}$  ( $\Omega_{vis} = 300$  meV) and  $I_{vis} = 7.1 \times 10^6 \mu\text{W} \cdot \mu\text{m}^{-2}$  ( $\Omega_{vis} = 3000$  meV). The dotted vertical gray lines indicate the fundamental frequency of vibrations A and B. (b): Evolution of the population of state  $|1, 0\rangle$  (left), state  $|0, 2\rangle$  (center) and state  $|0, 1\rangle$  (right) with the pumping laser intensity. Parameters:  $\hbar\omega_{vis} = \hbar\omega_{vis,1}^{cav} = 1.96$  eV,  $\hbar\kappa_{vis} = 160$  meV,  $\hbar\Omega_{vis}[\text{meV}] = 1.13\sqrt{I_{vis}[\mu\text{W} \cdot \mu\text{m}^{-2}]}$ ,  $\hbar\omega_A = 136$  meV,  $\hbar\omega_B = 68$  meV,  $\hbar g_F = 1.0$  meV,  $g_{vis,A} = 0.021$  meV,  $g_{vis,B} = 0.006$  meV,  $\gamma_A = \gamma_B = 1.2$  meV and  $T = 100$  K, Hilbert spaces with 3 number states for all the operators.

## S2. PUMP-PROBE CHARACTERIZATION OF IVR

In this section, we provide further detail on the modeling of the different pump-probe configurations for IVR characterization studied in Sections III.B, III.C and III.D of the main text. The accuracy of the models used is discussed and analytical insights are provided. The case of a Fermi resonance involving 3 vibrations ( $\omega_A \approx \omega_B + \omega_C$ ) is also studied for each configuration.

### A. Signatures of IVR under continuous-wave Stokes SERS pumping

#### 1. Fermi resonance with $\omega_A = 2\omega_B$

In this section, we discuss in more detail the analysis of IVR under continuous-wave SERS pumping and probing made in Section III.B of the main text. We consider the total Hamiltonian  $\hat{\mathcal{H}}_{tot}(t) = \hat{\mathcal{H}}_{vib,A} + \hat{\mathcal{H}}_{vib,B} + \hat{\mathcal{H}}_F + \hat{\mathcal{H}}_{vis}(t)$ , where the definitions of the  $\hat{\mathcal{H}}_{vib,i}$ , of  $\hat{\mathcal{H}}_F$  and of  $\hat{\mathcal{H}}_{vis}(t)$  are given in Eq. (1), Eq. (9) and Eq. (2) of the main text, respectively, and where  $\Omega_{vis}(t) = \Omega_{vis}^{cw}$  in  $\hat{\mathcal{H}}_{vis}$ . This Hamiltonian describes two molecular vibrations A and B coupled

between them by a Fermi resonance and coupled to an optical cavity by an optomechanical (Raman) interaction in SERS, and includes cavity pumping by a cw laser at visible frequencies. Following a similar approach and the same definitions as in Sections S1 A and S1 C, the total Hamiltonian can be cast into the time-independent form:

$$\begin{aligned}\hat{\mathcal{H}}_{tot} = & \hbar\omega_A\hat{b}_A^\dagger\hat{b}_A + \hbar\omega_B\hat{b}_B^\dagger\hat{b}_B + \hbar g_F(\hat{b}_A(\hat{b}_B^\dagger)^2 + \hat{b}_A^\dagger\hat{b}_B^2) + \hbar(\omega_{vis}^{cav} - \omega_{vis})\hat{a}_{vis}^\dagger\hat{a}_{vis} \\ & - \hbar g_{vis,A}|\alpha_{vis}|(\hat{a}_{vis}^\dagger + \hat{a}_{vis})(\hat{b}_A^\dagger + \hat{b}_A) - \hbar g_{vis,A}\hat{a}_{vis}^\dagger\hat{a}_{vis}(\hat{b}_A^\dagger + \hat{b}_A) \\ & - \hbar g_{vis,B}|\alpha_{vis}|(\hat{a}_{vis}^\dagger + \hat{a}_{vis})(\hat{b}_B^\dagger + \hat{b}_B) - \hbar g_{vis,B}\hat{a}_{vis}^\dagger\hat{a}_{vis}(\hat{b}_B^\dagger + \hat{b}_B).\end{aligned}\quad (S39)$$

According to Eq. (S4), the master equation of the system molecule-cavity is:

$$\partial_t \hat{\rho} = \frac{i}{\hbar} [\hat{\rho}(t), \hat{\mathcal{H}}_{tot}] + \frac{\kappa_{vis}}{2} \mathcal{D}_{\hat{a}_{vis}}[\hat{\rho}] + \sum_{i=A,B} \frac{\gamma_i(1+n_i^{th})}{2} \mathcal{D}_{\hat{b}_i}[\hat{\rho}] + \sum_{i=A,B} \frac{\gamma_i n_i^{th}}{2} \mathcal{D}_{\hat{b}_i^\dagger}[\hat{\rho}]. \quad (S40)$$

A first possibility to solve Eq. (S40) is to fully implement it with a numerical master equation solver. The black lines in Fig. S1 show calculations with this procedure of (a) the SERS spectra (using Eq. (S11)) and (b) the populations of the vibrational states ( $|1,0\rangle$ ,  $|0,2\rangle$ ,  $|0,1\rangle$ ), for the parameters given in Section III.A of the main text. The Python library QuTiP is used to solve the master equation [S26–S28]. We consider Hilbert spaces with 3 number states (i.e. states  $|0\rangle$ ,  $|1\rangle$ ,  $|2\rangle$ ) for the vibrations and (displaced) cavity operators, which we have verified gives accurate results for our system as long as cavity and vibrational populations remain typically  $\lesssim 0.1$ . The overall physical content of the figure is discussed in the main text.

A second option to solve Eq. (S40) is to introduce the linearization and adiabatic elimination of the operators of the visible cavity, as discussed in Section S1 A. Within these approximations, the master equation (S40) becomes:

$$\partial_t \hat{\rho}_{vib} = \frac{i}{\hbar} \left[ \hat{\rho}_{vib}, \sum_{i=A,B} \hbar\omega_i \hat{b}_i^\dagger \hat{b}_i + \hbar g_F(\hat{b}_A(\hat{b}_B^\dagger)^2 + \hat{b}_A^\dagger \hat{b}_B^2) \right] + \sum_{i=A,B} \frac{1}{2} [\gamma_i(1+n_i^{th}) + \Gamma_i^-] \mathcal{D}_{\hat{b}_i}[\hat{\rho}_{vib}] + \sum_{i=A,B} \frac{1}{2} [\gamma_i n_i^{th} + \Gamma_i^+] \mathcal{D}_{\hat{b}_i^\dagger}[\hat{\rho}_{vib}], \quad (S41)$$

where  $\hat{\rho}_{vib}$  is the reduced density matrix of the system composed of vibrations A and B. A vibrational coupling term  $\propto 2\hat{b}_A^\dagger \hat{\rho}_{vib} \hat{b}_B - \hat{b}_B \hat{b}_A^\dagger \hat{\rho}_{vib} - \hat{\rho}_{vib} \hat{b}_B \hat{b}_A^\dagger$  (and a corresponding term obtained by interchanging A and B) arise during the adiabatic elimination procedure, but are negligible as they involve vibrations with very different energies. The new master equation (S41) can again be solved numerically with QuTiP. The red dashed lines in Fig. S1 show calculations of the SERS spectra and populations (Fig. S1 (a) and Fig. S1 (b), respectively). The Hilbert spaces of the vibrations include again 3 number states for consistency with the previous option. We note that number states  $\gtrsim 10$  become accessible in this case due to the simplification of the master equation, which enables to check that all the results shown in Fig. S1 are already converged with 3 number states (not shown). Eqs. (S12),(S13) are used to calculate the SERS spectra. We now compare in Fig. S1 (a) calculations with this model (red dashed lines on the figure) and with the exact master equation (Eq. (S40), black lines). In the interval from -150 to -50 meV, which accounts for Stokes SERS by the vibrations, the agreement between the two models is very good for the two pumping strengths considered. By contrast, in the center (-50 to -50 meV) and anti-Stokes part (50 to 150 meV) of the spectrum, the background predicted by the full model (black lines) is significantly larger than for the model reduced to the vibrations (red lines). It is difficult to elucidate if this background is physical or is an artifact of the model. If physical, this background suggests that detecting signatures from very low populations may be challenging, particularly when also accounting for experimental noise in real-world setups. However, once the pumping power is large enough, Fig. S1 (a) shows that we can correctly reproduce the spectral features of interest, that are the anti-Stokes SERS peaks from the two vibrations. Furthermore, Fig. S1 (b) shows that a nearly perfect agreement is obtained for the populations of the various energy states. Therefore, the approximations introduced here are accurate (provided sufficient pumping strength for the spectra), enabling to solve the master equation of the system with a lower computational cost. This behavior justifies the use of the simplified model given by Eq. (S41) to obtain Figure 3 in the main text (obtained with the same value of the parameters as Fig. S1).

The third option to obtain the response of the system consists in an approximation of the master equation in Eq. (S41) to obtain analytical insights. In particular, the vibrational populations  $n_i(t) \equiv \langle \hat{b}_i^\dagger \hat{b}_i \rangle(t) \equiv \text{Tr}[\hat{b}_i^\dagger \hat{b}_i \hat{\rho}_{vib}(t)]$  obey the following set of equations:

$$\frac{dn_A}{dt} = -(\gamma_A + \Gamma_A^-)n_A + \Gamma_A^+(n_A + 1) + \gamma_A n_A^{th} + 2g_F \text{Im}[\langle \hat{b}_B^2 \hat{b}_A^\dagger \rangle], \quad (S42)$$

$$\frac{dn_B}{dt} = -(\gamma_B + \Gamma_B^-)n_B + \Gamma_B^+(n_B + 1) + \gamma_B n_B^{th} - 4g_F \text{Im}[\langle \hat{b}_B^2 \hat{b}_A^\dagger \rangle], \quad (S43)$$

$$\frac{d\langle \hat{b}_B^2 \hat{b}_A^\dagger \rangle}{dt} = - \left[ -i(\omega_A - 2\omega_B) + \frac{(\gamma_A + \Gamma_A^- - \Gamma_A^+ + 2\gamma_B + 2\Gamma_B^- - 2\Gamma_B^+)}{2} \right] \langle \hat{b}_B^2 \hat{b}_A^\dagger \rangle - ig_F(4\langle \hat{n}_B \hat{n}_A \rangle + 2n_A + n_B - \langle \hat{n}_B^2 \rangle), \quad (\text{S44})$$

$$\frac{d\langle \hat{n}_B^2 \rangle - n_B}{dt} = -2[\langle \hat{n}_B^2 \rangle - n_B] \times (\gamma_B + \Gamma_B^- - \Gamma_B^+) + 4n_B(\gamma_B n_B^{th} + \Gamma_B^+) - 4g_F \text{Im}[\langle \hat{b}_B^2 \hat{b}_A^\dagger \rangle + 2\langle \hat{n}_B \hat{b}_B^2 \hat{b}_A^\dagger \rangle], \quad (\text{S45})$$

where the origin of each term can be traced back to Eq. (S10) and Eqs. (S30-S32). In order to be solved, this set of equations needs to be closed. To this end, we introduce the approximations  $\langle \hat{n}_B \hat{n}_A \rangle \approx \langle \hat{n}_A \rangle \langle \hat{n}_B \rangle$  and  $\langle \hat{n}_B \hat{b}_B^2 \hat{b}_A^\dagger \rangle \approx \langle \hat{b}_B^2 \hat{b}_A^\dagger \rangle \langle \hat{n}_B \rangle$ , whose accuracy has been checked numerically. Consequently, given that  $n_B \ll 1$  in this work, we get  $\langle \hat{n}_B \hat{n}_A \rangle \ll n_A$  and  $\langle \hat{n}_B \hat{b}_B^2 \hat{b}_A^\dagger \rangle \ll \langle \hat{b}_B^2 \hat{b}_A^\dagger \rangle$ , so that  $\langle \hat{n}_B \hat{n}_A \rangle$  and  $\langle \hat{n}_B \hat{b}_B^2 \hat{b}_A^\dagger \rangle$  can be neglected in the equations (S42-S45). With these approximations, the set of equations (S42-S45) becomes closed and can be solved numerically in an efficient manner. This solution also provide directly the populations of the energy states in the subset  $\{|1, 0\rangle, |0, 2\rangle, |0, 1\rangle\}$ , by noting that  $n_A \approx n_{|1,0\rangle}$ ,  $\langle \hat{n}_B^2 \rangle - n_B \approx n_{|0,2\rangle}$  and  $2n_B - \langle \hat{n}_B^2 \rangle \approx n_{|0,1\rangle}$ . Under continuous-wave pumping, the states populations calculated with this procedure are shown as green dotted lines in Fig. S1 (b). These results are in perfect agreement with those obtained without approximations using Eq.(S40), which justifies the approximations introduced to close the set of equations (S42-S45). Finally, to obtain insights into the dynamics of the system, we combine Eq. (S43) with Eq.(S45) and obtain that the population of the fundamental of vibration B ( $|0, 1\rangle$ ) follows the dynamical equation:

$$\frac{dn_{|0,1\rangle}}{dt} \approx n_{|0,2\rangle}[\gamma_B(1 - 4n_B^{th}) + \Gamma_B^- - 5\Gamma_B^+] - n_{|0,1\rangle}[\gamma_B(1 + 4n_B^{th}) + \Gamma_B^- - 5\Gamma_B^+] + \gamma_B n_B^{th} + \Gamma_B^+. \quad (\text{S46})$$

On the one hand, Eq. (S46) shows that the Fermi resonance does not introduce any direct transfer from vibration A (state  $|1, 0\rangle$ ) to the fundamental of vibration B (state  $|0, 1\rangle$ ). Instead, the population is transferred from state  $|0, 2\rangle$  to state  $|0, 1\rangle$  by incoherent decay at rate  $n_{|0,2\rangle}[\gamma_B(1 - 4n_B^{th}) + \Gamma_B^- - 5\Gamma_B^+]$ . Additionally, the steady-state solution of Eq. (S46) results in  $n_{|0,1\rangle} \approx n_{|0,2\rangle} + n_B^{th} + \Gamma_B^+/\gamma_B$ , where  $\Gamma_B^+/\gamma_B$  corresponds to vibrational pumping by Stokes SERS (note that we have considered that  $n_B^{th} \ll 1$  and  $\Gamma_B^+, \Gamma_B^- \ll \gamma_B$ ). Hence, the population of state  $|0, 1\rangle$  is always greater than the population of state  $|0, 2\rangle$ , as observed in Fig. 3 (b) of the main text.

## 2. Fermi resonance with $\omega_A \approx \omega_B + \omega_C$

In the main text and until here in the supporting information, we have considered the case of Fermi resonances involving 2 vibrations. This choice reduces the number of energy states and of SERS peaks at play and thus simplifies the discussion and understanding of the underlying physics. However, as shown in Eq. (8) of the main text, Fermi resonances are third order processes with generic coupling Hamiltonian  $U_{A,B,C}^{(3)} \hat{q}_A \hat{q}_B \hat{q}_C$ , so that they can also involve three different vibrations ( $A \neq B \neq C$ ). This case is actually the most frequent in molecules [S29]. Furthermore, in a realistic molecule, the resonance condition  $\omega_A = \omega_B + \omega_C$  is unlikely to be perfectly fulfilled. In this section, we thus focus on the general case of a Fermi resonance involving 3 different vibrations that are not perfectly resonant, upon pumping by continuous-wave Stokes SERS and probing by cw anti-Stokes SERS (see Fig. S2 (a)). We find that Fermi resonances with  $\omega_A \approx \omega_B + \omega_C$  yield similar signatures of population transfer as those evidenced in the main text for Fermi resonances with  $\omega_A = 2\omega_B$ . The results obtained in this section thus strongly support the generality of our approach and indicate that SERS can be used to characterize IVR experimentally in a broad class of molecules.

We consider here that these three vibrations are coupled optomechanically to an optical cavity that is illuminated by a visible laser. Following a similar approach and the same definitions as in Sections S1A and S1C, the total Hamiltonian can be cast into the time-independent form:

$$\begin{aligned} \hat{\mathcal{H}}_{tot} = & \hbar\omega_A \hat{b}_A^\dagger \hat{b}_A + \hbar\omega_B \hat{b}_B^\dagger \hat{b}_B + \hbar\omega_C \hat{b}_C^\dagger \hat{b}_C + \hbar g_F (\hat{b}_A \hat{b}_B^\dagger \hat{b}_C^\dagger + \hat{b}_A^\dagger \hat{b}_B \hat{b}_C) + \hbar(\omega_{\text{vis}}^{\text{cav}} - \omega_{\text{vis}}) \hat{a}_{\text{vis}}^\dagger \hat{a}_{\text{vis}} \\ & - \hbar g_{\text{vis},A} |\alpha_{\text{vis}}| (\hat{a}_{\text{vis}}^\dagger + \hat{a}_{\text{vis}}) (\hat{b}_A^\dagger + \hat{b}_A) - \hbar g_{\text{vis},A} \hat{a}_{\text{vis}}^\dagger \hat{a}_{\text{vis}} (\hat{b}_A^\dagger + \hat{b}_A) \\ & - \hbar g_{\text{vis},B} |\alpha_{\text{vis}}| (\hat{a}_{\text{vis}}^\dagger + \hat{a}_{\text{vis}}) (\hat{b}_B^\dagger + \hat{b}_B) - \hbar g_{\text{vis},B} \hat{a}_{\text{vis}}^\dagger \hat{a}_{\text{vis}} (\hat{b}_B^\dagger + \hat{b}_B) \\ & - \hbar g_{\text{vis},C} |\alpha_{\text{vis}}| (\hat{a}_{\text{vis}}^\dagger + \hat{a}_{\text{vis}}) (\hat{b}_C^\dagger + \hat{b}_C) - \hbar g_{\text{vis},C} \hat{a}_{\text{vis}}^\dagger \hat{a}_{\text{vis}} (\hat{b}_C^\dagger + \hat{b}_C), \end{aligned} \quad (\text{S47})$$

where the Fermi resonance coupling strength is given by  $\hbar g_F = U_{A,B,C}^{(3)} q_A^0 q_B^0 q_C^0$ . Within this section, we consider that the three vibrations do not perfectly satisfy the resonance condition, i.e.  $\omega_A$  is similar but not identical to  $\omega_B + \omega_C$ .

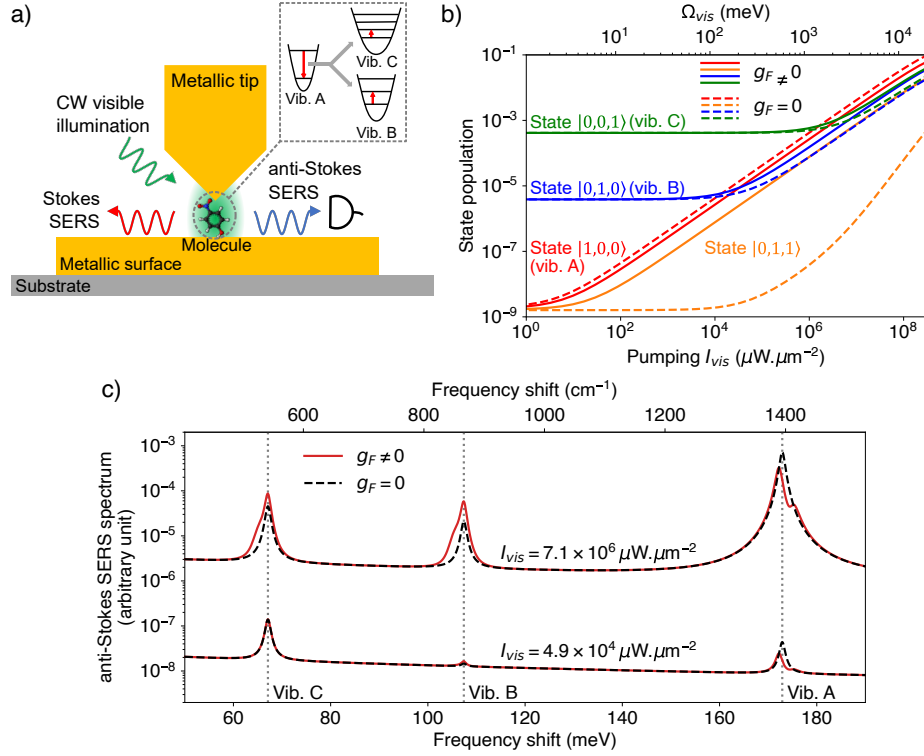

FIG. S2. Signatures of IVR under cw Stokes SERS pumping and anti-Stokes SERS probing for a Fermi resonance involving 3 vibrational modes. (a): sketch of the configuration under study, which consists in a single molecule in a single-mode plasmonic gap nanocavity resonant at 633 nm (mode 1 in Section II.A of the main text), resonantly illuminated with continuous-wave laser light (wavelength 633 nm, green arrow). The red arrow represents SERS emission by Stokes scattering processes, that also induces a pumping of the molecular vibrations. The blue arrow stands for the measured anti-Stokes SERS signal. (b): Evolution of the population of state  $|1,0,0\rangle$  (red continuous and dashed lines), state  $|0,1,1\rangle$  (orange lines), state  $|0,1,0\rangle$  (blue lines) and state  $|0,0,1\rangle$  (green lines) with the intensity of the pumping laser. The Fermi resonance coupling between vibrations A, B and C is included ( $g_F > 0$ , solid lines) or neglected ( $g_F = 0$ , dashed line). (c): anti-Stokes SERS spectra of the molecule with three vibrations coupled by the Fermi resonance (red lines) or uncoupled (black dashed lines), for two pumping intensities  $I_{\text{vis}} = 4.9 \times 10^4 \mu\text{W} \cdot \mu\text{m}^{-2}$  ( $\Omega_{\text{vis}} = 250$  meV) and  $I_{\text{vis}} = 7.1 \times 10^6 \mu\text{W} \cdot \mu\text{m}^{-2}$  ( $\Omega_{\text{vis}} = 3000$  meV). The dotted vertical gray lines indicate the fundamental frequency of vibrations A, B and C. Panels (b) and (c) are obtained using the model based on linearization and adiabatic elimination of the cavity degrees of freedom and with 3 number states for the Hilbert spaces of the molecular vibrations. Parameters:  $\hbar\omega_{\text{vis}} = \hbar\omega_{\text{vis},1}^{\text{cav}} = 1.96$  eV,  $\hbar\kappa_{\text{vis}} = 160$  meV,  $\hbar\Omega_{\text{vis}}[\text{meV}] = 1.13\sqrt{I_{\text{vis}}[\mu\text{W} \cdot \mu\text{m}^{-2}]}$ ,  $\hbar\omega_A = 172.9$  meV,  $\hbar\omega_B = 107.4$  meV,  $\hbar\omega_C = 67.1$  meV,  $\hbar g_F = 1.25$  meV,  $g_{\text{vis},A} = 0.024$  meV,  $g_{\text{vis},B} = 0.007$  meV,  $g_{\text{vis},C} = 0.006$  meV,  $\gamma_A = \gamma_B = \gamma_C = 1.2$  meV and  $T = 100$  K, Hilbert spaces with 2 number states for all the operators.

In addition, we use the same laser and cavity parameters as in Section II.B of the main text (i.e.  $\hbar\omega_{\text{vis}} = \hbar\omega_{\text{vis}}^{\text{cav}} = 1.96$  eV,  $\hbar\kappa_{\text{vis}} = 160$  meV and  $\hbar\Omega_{\text{vis}}[\text{meV}] = 1.13\sqrt{I_{\text{vis}}[\mu\text{W} \cdot \mu\text{m}^{-2}]}$ ). Further, we choose a Fermi resonance of the 4-nitrobenzenethiol molecule involving a mode A with frequency  $\hbar\omega_A = 172.9$  meV, a mode B with frequency  $\hbar\omega_B = 107.4$  meV and a mode C with frequency  $\hbar\omega_C = 67.1$  meV. These frequencies are estimated using DFT calculations of a NBT molecule bound to 19 atoms of gold (see Section S4). The same DFT calculations yield the estimate  $\hbar g_F = 1.25$  meV of Fermi resonance coupling strength and enable to calculate the Raman tensors of the vibrations. Inserting the latter values into Eq. (S3) yields the optomechanical coupling strengths  $g_{\text{vis},A} = 0.024$  meV for mode A,  $g_{\text{vis},B} = 0.007$  meV for mode B and  $g_{\text{vis},C} = 0.006$  meV for mode C. We use equal vibrational loss rates  $\gamma_A = \gamma_B = \gamma_C = 1.2$  meV for the three vibrations and assume operation at cryogenic molecular temperature  $T = 100$  K. Additionally, in this section, we focus our study on the subset of energy states of the vibrational system composed of the fundamental state of each vibrations ( $|1,0,0\rangle$  for vibration A,  $|0,1,0\rangle$  for vibration B and  $|0,0,1\rangle$  for vibration C), and of the state  $|0,1,1\rangle$  combining the fundamentals of vibration B and C. Finally, the master equation associated to the Hamiltonian (S47) has the same form as Eq. (S40), provided that sums over vibrations A and B are extended to vibration C.

We now study the signatures of IVR that can be observed on the vibrational populations and SERS spectra. Fig. S2 (c) shows the corresponding anti-Stokes SERS spectra obtained by including the coupling of the three vibrational

modes (red lines) for two visible pumping intensities  $I_{\text{vis}} = 4.9 \times 10^4 \text{ } \mu\text{W} \cdot \mu\text{m}^{-2}$  and  $I_{\text{vis}} = 7.1 \times 10^6 \text{ } \mu\text{W} \cdot \mu\text{m}^{-2}$ . Data calculated with  $g_F = 0$  are shown for reference (black dashed lines). Fig. S2 (b) shows the evolution of the population of the vibrational states with respect to illumination intensity  $I_{\text{vis}}$ , with ( $g_F > 0$ , continuous lines) or without ( $g_F = 0$ , dashed lines) the Fermi resonance. All data in Fig. S2 are obtained by solving a master equation in which the cavity degrees of freedom in the Hamiltonian Eq. (S47) are linearized and then adiabatically eliminated (more details are given below when comparing with other methodologies). Hilbert spaces with 3 number states for the 3 vibrations are used. The general trends displayed by the SERS spectra and the vibrational populations are the same as those discussed in the main text for Fermi resonances involving two vibrations. In particular, Fig. S2 (c) shows that for high illumination intensities ( $I_{\text{vis}} = 7.1 \times 10^6 \text{ } \mu\text{W} \cdot \mu\text{m}^{-2}$ ), the Fermi resonance induces a large enhancement of the anti-Stokes SERS signal emitted by the vibrations B and C (compare solid lines for  $g_F > 0$  with dashed lines for  $g_F = 0$ ). Panel (c) also shows that the peak around 172.9 meV associated to the Fermi resonance doublet is asymmetric (one peak of the doublet has a larger amplitude compared to the other), and that the peaks around 107.4 meV (associated to vibration B) and around 67.1 meV (associated to vibration C) present a shoulder, by contrast to the peaks seen in Fig. 3 (c) of the main text. These asymmetric features arise due to the frequency detuning between the vibrations, and it does not affect the possibility to observe the enhancement of the anti-Stokes SERS signal. Additionally, Fig. S2 (b) confirms that the population transfer by IVR remains large. For example, the population when the Fermi coupling is included (continuous green line) is  $1.8 \times$  larger than when  $g_F = 0$  (dashed green line) in the range  $I_{\text{vis}} = 10^7 - 10^8 \text{ } \mu\text{W} \cdot \mu\text{m}^{-2}$ , in spite of the sizable frequency detuning between the vibrations  $\hbar|\omega_A - \omega_B - \omega_C| = 1.6 \text{ meV} > \hbar\gamma_A, \hbar\gamma_B, \hbar\gamma_C$ . In summary, Fig. S2 shows that conclusions equivalent to those presented in Section II. B of the main text can be drawn for Fermi resonances involving 3 vibrations.

To verify the validity of different simplifications and provide strategies to reduce the computational cost of the simulations, we discuss next several options to obtain the vibrational populations and SERS spectra for Fermi resonances involving 3 vibrations under cw visible illumination of the optical cavity. A first option is to solve the full master equation associated to the Hamiltonian in Eq. (S47). The black lines in Fig. S3 show calculations of the Raman spectra (panel (a)) and vibrational population (panel (b)) with this procedure using QuTiP and Hilbert spaces with 2 number states for the cavity and vibrations operators. We use 2 number states, instead of 3 in the previous case of a  $\omega_A = 2\omega_B$  Fermi resonance, because introducing a third vibration in the present case severely increases the computation time. A second option is to consider the linearization and adiabatic elimination of the cavity degrees of freedom approximations introduced in Section S1 A, which yields a simplified master equation similar to Eq. (S41). The red dashed lines in Fig. S3 show calculations with this procedure using QuTiP and Hilbert spaces with 2 number states for the vibrations operators. We have verified that increasing the number of number states in these calculations do not modify the results. Finally, for the calculation of the vibrational populations, the simplified master equation also allows to obtain a closed set of differential equations:

$$\frac{dn_A}{dt} = -(\gamma_A + \Gamma_A^-)n_A + \Gamma_A^+(n_A + 1) + \gamma_A n_A^{th} + 2g_F \text{Im}[\langle \hat{b}_A^\dagger \hat{b}_B \hat{b}_C \rangle], \quad (\text{S48})$$

$$\frac{dn_B}{dt} = -(\gamma_B + \Gamma_B^-)n_B + \Gamma_B^+(n_B + 1) + \gamma_B n_B^{th} - 2g_F \text{Im}[\langle \hat{b}_A^\dagger \hat{b}_B \hat{b}_C \rangle], \quad (\text{S49})$$

$$\frac{dn_C}{dt} = -(\gamma_C + \Gamma_C^-)n_C + \Gamma_C^+(n_C + 1) + \gamma_C n_C^{th} - 2g_F \text{Im}[\langle \hat{b}_A^\dagger \hat{b}_B \hat{b}_C \rangle], \quad (\text{S50})$$

$$\begin{aligned} \frac{d\langle \hat{b}_A^\dagger \hat{b}_B \hat{b}_C \rangle}{dt} = & - \left[ -i(\omega_A - \omega_B - \omega_C) + \frac{(\gamma_A + \Gamma_A^- - \Gamma_A^+ + \gamma_B + \Gamma_B^- - \Gamma_B^+ + \gamma_C + \Gamma_C^- - \Gamma_C^+)}{2} \right] \langle \hat{b}_A^\dagger \hat{b}_B \hat{b}_C \rangle \\ & - ig_F [n_A(1 + n_B + n_C) - \langle \hat{n}_B \hat{n}_C \rangle], \end{aligned} \quad (\text{S51})$$

$$\begin{aligned} \frac{d\langle \hat{n}_B \hat{n}_C \rangle}{dt} = & -(\gamma_B + \Gamma_B^- - \Gamma_B^+ + \gamma_C + \Gamma_C^- - \Gamma_C^+) \langle \hat{n}_B \hat{n}_C \rangle + (\gamma_B n_B^{th} + \Gamma_B^+)n_C + (\gamma_C n_C^{th} + \Gamma_C^+)n_B \\ & - 2g_F \text{Im}[\langle \hat{b}_A^\dagger \hat{b}_B \hat{b}_C \rangle] (1 + n_B + n_C). \end{aligned} \quad (\text{S52})$$

where the approximations  $\langle \hat{n}_A \hat{n}_B \rangle \rightarrow n_A n_B$ ,  $\langle \hat{n}_A \hat{n}_C \rangle \rightarrow n_A n_C$ ,  $\langle \hat{n}_B \hat{b}_A^\dagger \hat{b}_B \hat{b}_C \rangle \rightarrow n_B \langle \hat{b}_A^\dagger \hat{b}_B \hat{b}_C \rangle$  and  $\langle \hat{n}_C \hat{b}_A^\dagger \hat{b}_B \hat{b}_C \rangle \rightarrow n_C \langle \hat{b}_A^\dagger \hat{b}_B \hat{b}_C \rangle$  have been introduced (see Section S2 A 1 for more details). A numerical implementation of this third option is shown as green dotted lines in Fig. S3 (b). We now compare the simulations obtained with the various

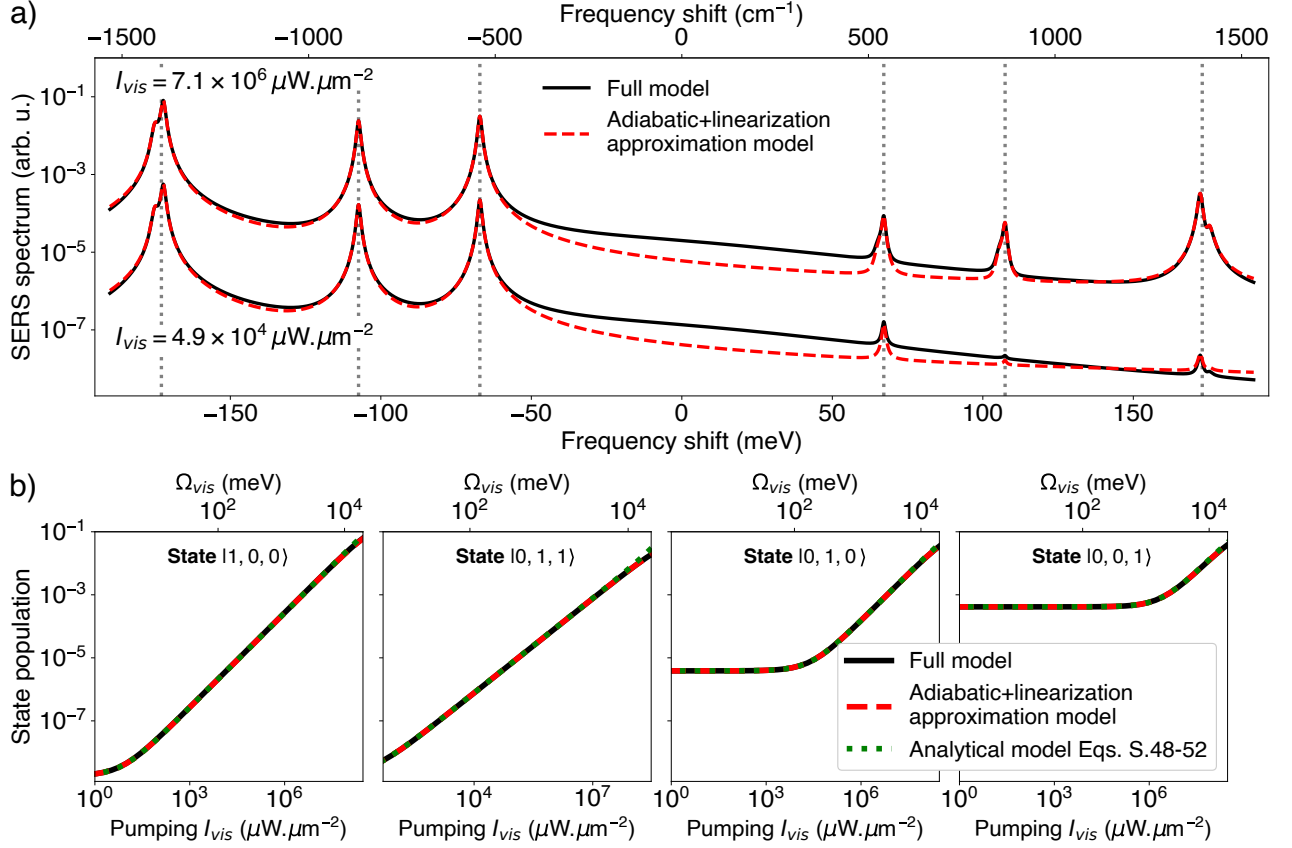

FIG. S3. Comparison of models used to analyze the importance of IVR under cw Stokes SERS pumping and cw anti-Stokes SERS probing for Fermi resonances involving 3 vibrational modes. Black continuous lines show results obtained by solving the master equation based on the full Hamiltonian in Eq. (S47). Red dashed lines are obtained by solving a master equation in which the cavity degrees of freedom have been linearized and adiabatically eliminated. These results are the same as in Fig. S2. The green dotted lines in panel (b) correspond to solutions of the set of approximated equations (S48-S52). (a): anti-Stokes SERS spectra for two pumping intensities  $I_{\text{vis}} = 4.9 \times 10^4 \mu\text{W} \cdot \mu\text{m}^{-2}$  ( $\Omega_{\text{vis}} = 250 \text{ meV}$ ) and  $I_{\text{vis}} = 7.1 \times 10^6 \mu\text{W} \cdot \mu\text{m}^{-2}$  ( $\Omega_{\text{vis}} = 3000 \text{ meV}$ ). The dotted vertical gray lines indicate the fundamental frequency of vibrations A, B and C. (b): Evolution of the population of state  $|1, 0, 0\rangle$  (left), state  $|0, 1, 1\rangle$  (center left), state  $|0, 1, 0\rangle$  (center right) and state  $|0, 0, 1\rangle$  (right) with the intensity of the pumping laser. Parameters:  $\hbar\omega_{\text{vis}} = \hbar\omega_{\text{vis},1}^{\text{cav}} = 1.96 \text{ eV}$ ,  $\hbar\kappa_{\text{vis}} = 160 \text{ meV}$ ,  $\hbar\Omega_{\text{vis}}[\text{meV}] = 1.13\sqrt{I_{\text{vis}}[\mu\text{W} \cdot \mu\text{m}^{-2}]}$ ,  $\hbar\omega_A = 172.9 \text{ meV}$ ,  $\hbar\omega_B = 107.4 \text{ meV}$ ,  $\hbar\omega_C = 67.1 \text{ meV}$ ,  $\hbar g_F = 1.25 \text{ meV}$ ,  $g_{\text{vis},A} = 0.024 \text{ meV}$ ,  $g_{\text{vis},B} = 0.007 \text{ meV}$ ,  $g_{\text{vis},C} = 0.006 \text{ meV}$ ,  $\gamma_A = \gamma_B = \gamma_C = 1.2 \text{ meV}$  and  $T = 100 \text{ K}$ , Hilbert spaces with 2 number states for all the operators. The dashed red lines in the figure correspond to the case  $g_F \neq 0$  in Fig. S2 (except for the different ranges of values).

models. In Fig. S3 (a), the agreement between the full model and the model based on linearization and adiabatic elimination in the Stokes (-200 to -50 meV) part of the spectrum is nearly perfect in the two pumping cases. In the center (-50 to 50 meV) and anti-Stokes (50 to 200 meV) part of the spectrum, we recover the larger background for the full model discussed in the previous section. For the low excitation intensity  $I_{\text{vis}} = 4.9 \times 10^4 \mu\text{W} \cdot \mu\text{m}^{-2}$ , as the amplitude of the anti-Stokes SERS peaks is low compared to the background, notable discrepancies between the two models are observable. In addition, this suggests that for low excitation intensities and low temperatures, the anti-Stokes SERS peaks may be difficult to identify in experimental measurements. Nevertheless, the traces in Fig. S3 (a) with  $I_{\text{vis}} = 7.1 \times 10^6 \mu\text{W} \cdot \mu\text{m}^{-2}$  show that once higher pumping intensities are considered, a large signal-to-noise ratio can be reached. When achieved, the figure further shows that a very good agreement is reached between the two models for the anti-Stokes SERS peaks, which are the signals of interest for the characterization techniques of IVR considered in this work. On the other hand, Fig. S3 (b) show the evolution of the states population with intensity, for which a nearly perfect agreement is reached between the three models. Therefore, the model based on linearization and adiabatic elimination is as a convenient alternative to the full model in the pumping regimes where the effect of IVR is significant, as it requires lower computational resources. For the vibrational populations, the semi-analytical model based on Eqs. (S48-S52) can also be used.

## B. Transient signatures of IVR under pulsed Stokes SERS pumping

In this section of the SI, we examine in more detail the transient signatures of an individual IVR pathway that can be observed under pulsed pumping and probing with visible light. We first focus on a Fermi resonance with  $\omega_A = 2\omega_B$ , and provide more details about the model used to obtain the results presented in Section III.C of the main text. We then analyze and discuss the more general case of a Fermi resonance with  $\omega_A \approx \omega_B + \omega_C$ .

### 1. Fermi resonance with $\omega_A = 2\omega_B$

In Section III.C of the main text, we consider an optical cavity supporting two modes in the visible range, respectively at frequency  $\omega_{\text{VIS},1}^{\text{CAV}} = 1.96$  eV (i.e 633 nm, noted mode 1) and  $\omega_{\text{VIS},2}^{\text{CAV}} = 1.58$  eV (i.e. 785 nm, mode 2), and the total Hamiltonian  $\hat{\mathcal{H}}_{\text{tot}}(t-t^{\text{probe}}) = \hat{\mathcal{H}}_{\text{VIB},A} + \hat{\mathcal{H}}_{\text{VIB},B} + \hat{\mathcal{H}}_F + \hat{\mathcal{H}}_{\text{VIS}}^{\text{pump}}(t) + \hat{\mathcal{H}}_{\text{VIS}}^{\text{probe}}(t-t^{\text{probe}})$  where  $\hat{\mathcal{H}}_{\text{VIB},i}$  accounts for the energy of the vibration  $i$  (see Eq. (1) of the main text),  $\hat{\mathcal{H}}_F$  for the coupling of the two vibrations by a Fermi resonance (see Eq. (9) of the main text),  $\hat{\mathcal{H}}_{\text{VIS}}^{\text{pump}}(t)$  for a pulse of light tuned to the cavity mode 2 ( $\omega_{\text{VIS}}^{\text{pump}} = \omega_{\text{VIS},2}^{\text{CAV}}$ ) and centered at time  $t = 0$  that induces pumping of the vibrations by Stokes SERS (see Eq. (2) of the main text), and  $\hat{\mathcal{H}}_{\text{VIS}}^{\text{probe}}(t-t^{\text{probe}})$  for a pulse of light tuned to the cavity mode 1 ( $\omega_{\text{VIS}}^{\text{probe}} = \omega_{\text{VIS},1}^{\text{CAV}}$ ) and centered at time  $t^{\text{probe}}$  that serves to probe the population of the vibrations by inducing anti-Stokes SERS. The envelop of the pulses are considered as Gaussian, with  $\Omega_{\text{VIS}}^{\text{pump}}(t) = \Omega_{\text{VIS}}^{\text{pump,max}} e^{-2 \ln(2) \times [t/\Delta\tau^{\text{pump}}]^2}$  in  $\hat{\mathcal{H}}_{\text{VIS}}^{\text{pump}}(t)$  and  $\Omega_{\text{VIS}}^{\text{probe}}(t-t^{\text{probe}}) = \Omega_{\text{VIS}}^{\text{probe,max}} e^{-2 \ln(2) \times [(t-t^{\text{probe}})/\Delta\tau^{\text{probe}}]^2}$  in  $\hat{\mathcal{H}}_{\text{VIS}}^{\text{probe}}(t-t^{\text{probe}})$ , where  $\Omega_{\text{VIS}}^{\text{pump,max}}$  and  $\Omega_{\text{VIS}}^{\text{probe,max}}$  are the amplitudes of the envelopes, and  $\Delta\tau^{\text{pump}}$  and  $\Delta\tau^{\text{probe}}$  are the pulses duration (defined as the total time for which the intensity of the pulses is larger than half of the maximum intensity). Following a similar approach and the same definitions as in Sections S1 A and S1 C, the total Hamiltonian can be cast into the form:

$$\begin{aligned} \hat{\mathcal{H}}_{\text{tot}}(t) = & \hbar\omega_A \hat{b}_A^\dagger \hat{b}_A + \hbar\omega_B \hat{b}_B^\dagger \hat{b}_B + \hbar g_F (\hat{b}_A (\hat{b}_B^\dagger)^2 + \hat{b}_A^\dagger \hat{b}_B^2) \\ & + \hbar(\omega_{\text{VIS},1}^{\text{CAV}} - \omega_{\text{VIS}}^{\text{probe}}) \hat{a}_{\text{VIS},1}^\dagger \hat{a}_{\text{VIS},1} + \hbar(\omega_{\text{VIS},2}^{\text{CAV}} - \omega_{\text{VIS}}^{\text{pump}}) \hat{a}_{\text{VIS},2}^\dagger \hat{a}_{\text{VIS},2} \\ & - \sum_{i=A,B} \hbar g_{\text{VIS},i} |\alpha_{\text{VIS}}^{\text{pump}}(t)| (\hat{a}_{\text{VIS},2}^\dagger + \hat{a}_{\text{VIS},2}) (\hat{b}_i^\dagger + \hat{b}_i) - \hbar g_{\text{VIS},i} \hat{a}_{\text{VIS},2}^\dagger \hat{a}_{\text{VIS},2} (\hat{b}_i^\dagger + \hat{b}_i) \\ & - \sum_{i=A,B} \hbar g_{\text{VIS},i} |\alpha_{\text{VIS}}^{\text{probe}}(t-t^{\text{probe}})| (\hat{a}_{\text{VIS},1}^\dagger + \hat{a}_{\text{VIS},1}) (\hat{b}_i^\dagger + \hat{b}_i) - \hbar g_{\text{VIS},i} \hat{a}_{\text{VIS},1}^\dagger \hat{a}_{\text{VIS},1} (\hat{b}_i^\dagger + \hat{b}_i), \end{aligned} \quad (\text{S53})$$

where  $\alpha_{\text{VIS}}^{\text{pump}}(t)$ ,  $\alpha_{\text{VIS}}^{\text{probe}}(t-t^{\text{probe}})$  are written as  $\alpha_{\text{VIS}}^{\text{pump}}(t) = \Omega_{\text{VIS}}^{\text{pump}}(t)/[i(\omega_{\text{VIS},2}^{\text{CAV}} - \omega_{\text{VIS}}^{\text{pump}}) + \kappa_{\text{VIS}}/2]$  and  $\alpha_{\text{VIS}}^{\text{probe}}(t-t^{\text{probe}}) = \Omega_{\text{VIS}}^{\text{probe}}(t-t^{\text{probe}})/[i(\omega_{\text{VIS},1}^{\text{CAV}} - \omega_{\text{VIS}}^{\text{probe}}) + \kappa_{\text{VIS}}/2]$ . We note that these later expressions are derived for continuous-wave illumination (see Sec. S1 A), but can be used under pulsed illumination as long as  $\alpha_{\text{VIS}}$  follows adiabatically the variations of  $\Omega_{\text{VIS}}$ . To this end, the temporal variations of  $\omega_{\text{VIS}}^{\text{pump}}$  and  $\omega_{\text{VIS}}^{\text{probe}}$  with time  $t$  must be slow compared to the cavity photon residence time, i.e.  $|\partial_t \Omega_{\text{VIS}}^{\text{pump/probe}}|(t) \ll \kappa_{\text{VIS}} \Omega_{\text{VIS}}^{\text{pump/probe,max}}$ , which is satisfied for the Gaussian pulses and the values  $\Delta\tau^{\text{pump/probe}} \geq 400$  fs,  $\hbar\kappa_{\text{VIS}} = 160$  meV considered in this work (in particular,  $\Delta\tau^{\text{pump/probe}} = 500$  fs is used in Section III.C of the main text). In addition, time-dependent terms  $\propto \hat{a}_{\text{VIS},2}^\dagger \hat{a}_{\text{VIS},1}$  and  $\propto \hat{a}_{\text{VIS},1}^\dagger \hat{a}_{\text{VIS},2}$  should in principle appear in the SERS coupling Hamiltonian when considering 2 cavity modes simultaneously (as the cavity electric field decompose on all the cavity modes  $\hat{\mathbf{E}} = \mathbf{E}_{\text{VIS},1}^{\text{CAV}} (\hat{a}_{\text{VIS},1} + \hat{a}_{\text{VIS},1}^\dagger) + \mathbf{E}_{\text{VIS},2}^{\text{CAV}} (\hat{a}_{\text{VIS},2} + \hat{a}_{\text{VIS},2}^\dagger)$  and the SERS coupling Hamiltonian is  $\propto \hat{\mathbf{E}}^2$  [S2]). However, these terms are neglected in Eq. (S53) due to the large frequency detuning between cavity modes 1 and 2 (i.e.  $\omega_{\text{VIS},1}^{\text{CAV}} - \omega_{\text{VIS},2}^{\text{CAV}} > 2\kappa_{\text{VIS}}$ ), which causes them to oscillate rapidly so that their contribution averages out when solving the master equation.

The master equation corresponding to the Hamiltonian given in Eq. (S53) can be directly solved numerically. However, in order to reduce the computation time, we resort in this section to the linearization and adiabatic elimination of the cavity modes degrees of freedom introduced in Section S1 A. These approximations have been shown to accurately reproduce the Raman peaks and vibrational populations in presence of a Fermi resonance in Section S2 A. Within these approximations, the master equation of the density matrix  $\hat{\rho}_{\text{VIB}}$  reduced to the vibrational modes A and

B becomes:

$$\begin{aligned} \partial_t \hat{\rho}_{\text{VIB}} = & \frac{i}{\hbar} \left[ \hat{\rho}_{\text{VIB}}(t), \sum_{i=A,B} \hbar \omega_i \hat{b}_i^\dagger \hat{b}_i + \hbar g_F (\hat{b}_A (\hat{b}_B^\dagger)^2 + \hat{b}_A^\dagger \hat{b}_B^2) \right] \\ & + \sum_{i=A,B} \frac{1}{2} [\gamma_i (1 + n_i^{th}) + \Gamma_{1,i}^-(t - t^{\text{probe}}) + \Gamma_{2,i}^-(t)] \mathcal{D}_{\hat{b}_i} [\hat{\rho}_{\text{VIB}}] + \sum_{i=A,B} \frac{1}{2} [\gamma_i n_i^{th} + \Gamma_{1,i}^+(t - t^{\text{probe}}) + \Gamma_{2,i}^+(t)] \mathcal{D}_{\hat{b}_i^\dagger} [\hat{\rho}_{\text{VIB}}], \end{aligned} \quad (\text{S54})$$

where:

$$\Gamma_{1,i}^\pm(t - t^{\text{probe}}) = \frac{|\alpha_{\text{VIS}}^{\text{probe}}(t - t^{\text{probe}})|^2 g_{\text{VIS},i}^2 \kappa_{\text{VIS}}}{(\omega_{\text{VIS}}^{\text{probe}} \mp \omega_i - \omega_{\text{VIS},1}^{\text{cav}})^2 + (\kappa_{\text{VIS}}/2)^2} \quad \text{and} \quad \Gamma_{2,i}^\pm(t) = \frac{|\alpha_{\text{VIS}}^{\text{pump}}(t)|^2 g_{\text{VIS},i}^2 \kappa_{\text{VIS}}}{(\omega_{\text{VIS}}^{\text{pump}} \mp \omega_i - \omega_{\text{VIS},2}^{\text{cav}})^2 + (\kappa_{\text{VIS}}/2)^2}. \quad (\text{S55})$$

We now comment further on the quantity  $I_i^{\text{aS,int}}(t^{\text{probe}})$  plotted Fig. 4 (b) of the main text. Experimentally, it is possible to measure the anti-Stokes SERS spectra corresponding to a given probe pulse centered at time  $t^{\text{probe}}$ . Quantitatively, the measured quantity is thus:

$$I(\omega, t^{\text{probe}}) \propto \int_{-\infty}^{\infty} dt I^{0,t^{\text{probe}}}(\omega, t) dt, \quad (\text{S56})$$

where  $I^{0,t^{\text{probe}}}(\omega, t)$  is the SERS spectrum defined in Eq. (S11), in which the superscript  $0, t^{\text{probe}}$  indicates that illumination is achieved with a pump pulse centered at time 0 and a probe pulse centered at time  $t^{\text{probe}}$ . It is further possible to separate the anti-Stokes signals from vibrations A and B by integrating over the frequency region around their corresponding peaks. This yields the anti-Stokes SERS signal from a molecular vibration  $i$ , noted  $I_i^{\text{aS,int}}(t^{\text{probe}})$ , and formally defined as:

$$I_i^{\text{aS,int}}(t^{\text{probe}}) \propto \int_{\omega_i - \Delta}^{\omega_i + \Delta} d\omega \int_{-\infty}^{\infty} dt I^{0,\text{pr}}(\omega, t), \quad (\text{S57})$$

where  $\Delta$  is of the order of a few vibrational linewidth. For simplicity, in our theoretical approach, we use the approximated expression Eq. (S16) to calculate the SERS spectra, instead of the more rigorous Eq. (S11). With this assumption,  $I_i^{\text{aS,int}}(t^{\text{probe}})$  can be expressed as:

$$I_i^{\text{aS,int}}(t^{\text{probe}}) \propto (\omega_{\text{VIS},1}^{\text{cav}} + \omega_i)^4 \int_{-\infty}^{+\infty} \Gamma_{1,i}^-[\Omega_{\text{VIS}}^{\text{probe}}(t - t^{\text{probe}})] n_i^{0,t^{\text{probe}}}(t) dt, \quad (\text{S58})$$

where  $n_i^{0,t^{\text{probe}}}$  is the population of vibration  $i$  for a pump pulse centered at time  $t = 0$  and a probe pulse centered at time  $t^{\text{probe}}$ . The expression Eq. (S58) is the one used in Sec. III.C of the main text. In the simulations of Fig. 4 (b), the evolution of  $\hat{\rho}_{\text{VIB}}$  in Eq. (S54) is calculated in the time interval  $t \in [-3000, 7000]$  fs for each value of  $t^{\text{probe}}$  (which takes values from -1500 to 5000 fs). We then obtain the vibrational populations  $n_i^{0,t^{\text{probe}}}(t)$  for each time  $t$  in the time interval and use it to calculate Eq. (S58).

Finally, we emphasize that the set of equations (S42-S45) derived for a single cavity mode in Section S2 A also holds in this case provided the substitution  $\Gamma_i^\pm \rightarrow \Gamma_{1,i}^\pm(t) + \Gamma_{2,i}^\pm(t)$ . We have checked (not shown) that this approach results in a reasonable agreement with the results obtained by solving numerically Eq. (S54) and Eq. (S58), for the parameters used in Fig. 4 of the main text.

## 2. Fermi resonance with $\omega_A \approx \omega_B + \omega_C$

In this section, we analyze the possibility to identify IVR using pulsed SERS pumping and probing in the case of a Fermi resonance involving 3 different molecular vibrational modes A, B and C with a non-perfect resonance condition  $\omega_A \approx \omega_B + \omega_C$ . As in the previous section, we linearize the Hamiltonian and use the adiabatic elimination of the cavity degrees of freedom. The master equation for the density matrix reduced to the vibrational modes A, B and C then reads:

$$\begin{aligned} \partial_t \hat{\rho}_{\text{VIB}} = & \frac{i}{\hbar} \left[ \hat{\rho}_{\text{VIB}}(t), \sum_{i=A,B,C} \hbar \omega_i \hat{b}_i^\dagger \hat{b}_i + \hbar g_F (\hat{b}_A \hat{b}_B^\dagger \hat{b}_C^\dagger + \hat{b}_A^\dagger \hat{b}_B \hat{b}_C) \right] \\ & + \sum_{i=A,B,C} \frac{1}{2} [\gamma_i (1 + n_i^{th}) + \Gamma_{1,i}^-(t - t^{\text{probe}}) + \Gamma_{2,i}^-(t)] \mathcal{D}_{\hat{b}_i} [\hat{\rho}_{\text{VIB}}] + \sum_{i=A,B,C} \frac{1}{2} [\gamma_i n_i^{th} + \Gamma_{1,i}^+(t - t^{\text{probe}}) + \Gamma_{2,i}^+(t)] \mathcal{D}_{\hat{b}_i^\dagger} [\hat{\rho}_{\text{VIB}}], \end{aligned} \quad (\text{S59})$$

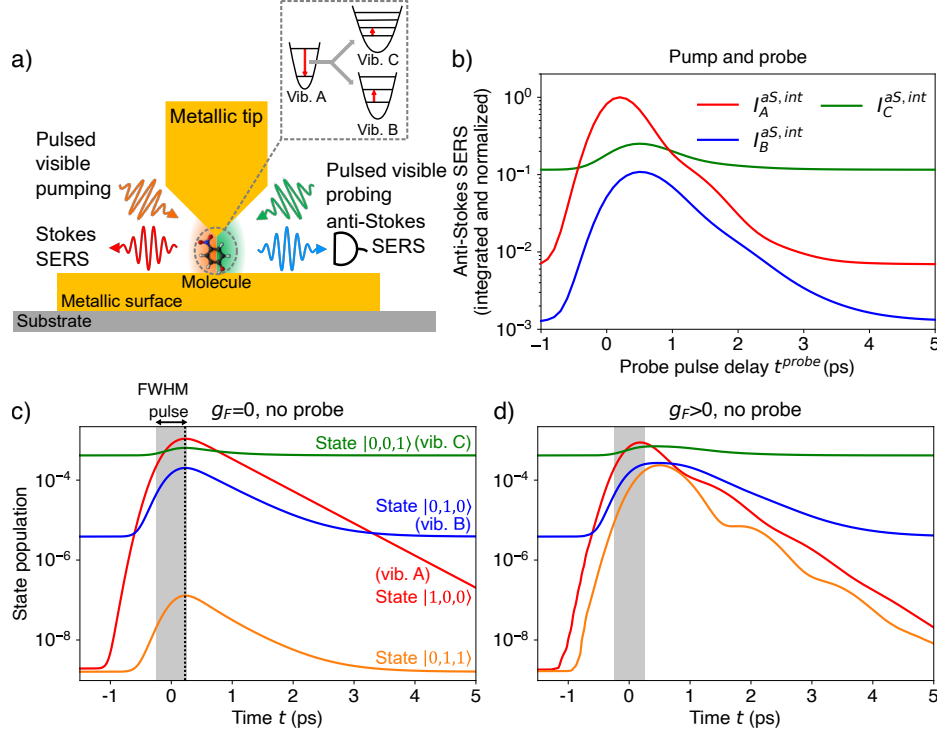

FIG. S4. *Signatures of IVR under pulsed Stokes SERS pumping and pulsed anti-Stokes SERS probing for a Fermi resonance involving 3 vibrational modes.* (a): Sketch of the configuration under study, which consists in a single molecule in a plasmonic gap nanocavity that supports two modes in the visible range, one resonant at 633 nm (alluded schematically by the green shadowing on the figure, corresponding to mode 1 in Section III. A of the main text) and another resonant at 785 nm (orange shadowing on the figure, mode 2 in Section III. A of the main text). The mode at 785 nm is resonantly illuminated with pulsed light (left orange arrow, pulse center at time 0) that produces Stokes SERS light (red arrow) and vibrational pumping of the molecular vibrations. The cavity mode at 633 nm is resonantly illuminated with pulsed light (right green arrow) that arrives at a delayed time  $t^{\text{probe}}$  and generates the measured anti-Stokes SERS signal (blue arrow). (b): Time dynamics of the integrated anti-Stokes SERS signals from vibrations A, B and C,  $I_A^{\text{aS,int}}(t)$  (red line),  $I_B^{\text{aS,int}}(t)$  (blue line) and  $I_C^{\text{aS,int}}(t)$  (green line), respectively. All curves are normalized to the maximum of  $I_A^{\text{aS,int}}(t)$ . (c): Dynamics of the population of the states  $|1,0,0\rangle$  (red line),  $|0,1,1\rangle$  (orange line),  $|0,1,0\rangle$  (blue line) and  $|0,0,1\rangle$  (green line) without probe pulse ( $\Omega_{\text{vis}}^{\text{probe,max}} = 0$ ) and without Fermi resonance coupling ( $g_F = 0$ ). The vertical black dotted line indicates the time  $\approx 230$  fs at which all the states roughly reach their maximum population. The gray shaded area indicate the time interval during which the pump pulse intensity is greater than half its peak value. (d): Same as in (c) but when the Fermi resonance coupling  $g_F > 0$  is included. Panels (b-d) are obtained using the model based on linearization and adiabatic elimination of the cavity degrees of freedom and with 3 number states for the Hilbert spaces of the molecular vibrations. Parameters: in all panels the Gaussian pump pulse duration has a full-width at half maximum (of intensity)  $\Delta\tau^{\text{pump}} = 500$  fs and a peak intensity  $I_{\text{vis}}^{\text{pump,max}} = 5.7 \times 10^6 \mu\text{W} \cdot \mu\text{m}^{-2}$  (i.e.  $\Omega_{\text{vis}}^{\text{pump,max}} = 3000$  meV). The Gaussian probe pulse is turned on in (b) with duration  $\Delta\tau^{\text{probe}} = 400$  fs and peak intensity  $I_{\text{vis}}^{\text{probe,max}} = 4.9 \times 10^4 \mu\text{W} \cdot \mu\text{m}^{-2}$  (i.e.  $\Omega_{\text{vis}}^{\text{probe,max}} = 250$  meV), and is turned off ( $I_{\text{vis}}^{\text{probe,max}} = 0$ ) in (c),(d). Other parameters:  $\hbar\omega_{\text{vis}}^{\text{pump}} = \hbar\omega_{\text{vis},2}^{\text{cav}} = 1.96$  eV,  $\hbar\omega_{\text{vis}}^{\text{probe}} = \hbar\omega_{\text{vis},1}^{\text{cav}} = 1.58$  eV,  $\hbar\kappa_{\text{vis}} = 160$  meV,  $\hbar\omega_A = 172.9$  meV,  $\hbar\omega_B = 107.4$  meV,  $\hbar\omega_C = 67.1$  meV,  $\hbar g_F = 1.25$  meV,  $\gamma_A = \gamma_B = \gamma_C = 1.2$  meV and  $T = 100$  K. In cavity mode 1:  $g_{\text{vis},A} = 0.024$  meV,  $g_{\text{vis},B} = 0.007$  meV,  $g_{\text{vis},C} = 0.006$  meV. In cavity mode 2:  $g_{\text{vis},A} = 0.020$  meV,  $g_{\text{vis},B} = 0.006$  meV,  $g_{\text{vis},C} = 0.005$  meV. The calculations comprise Hilbert spaces with 3 number states for the vibrational operators.

where the various quantities involved in the equation are defined in Sections S1 A and S2 B 1. Fig. S4 shows the dynamics of the integrated anti-Stokes SERS signals for the three vibrations  $I_i^{\text{aS,int}}$  (panel (b)) and, to specifically focus on the effect on pumping, of the dynamics of the states population when the Fermi resonance is turned on (panel (c)) and off (panel (d)). Similarly to the analysis made in Section III.C of the main text for the case of a Fermi resonance with  $\omega_A = 2\omega_B$ , a comparison of panels (c) and (d) evidences two signatures of the Fermi resonance coupling on the vibrational populations: (i) the presence of Rabi-like oscillations between the fundamental of vibration A (state  $|1,0,0\rangle$ , red line on the figure) and the combination of vibrations B and C (state  $|0,1,1\rangle$ , orange line), and (ii) a delayed non-equilibrium population of the fundamentals of vibrations B (state  $|0,1,0\rangle$ , blue line) and C (state  $|0,0,1\rangle$ , green line) compared to the case with no Fermi coupling. In addition, Fig. S4 (b) shows, on the one hand,

that the maxima of  $I_B^{\text{aS,int}}(t^{\text{probe}})$  and  $I_C^{\text{aS,int}}(t^{\text{probe}})$  are delayed by several hundred of femtosecond with respect to the center of the pump pulse (i.e. to  $t^{\text{probe}} = 0$  fs), so that the signature (ii) is likely to be identifiable in a realistic SERS experiment. On the other hand, Fig. S4 (b) also shows that the shoulder in  $I_A^{\text{aS,int}}(t^{\text{probe}})$  (continuous red line) corresponding to the Rabi oscillations can be observed for a probe pulse duration of 400 fs. Here, we use a slightly shorter probe pulse duration of 400 fs, against 500 fs in the main text. This is because the probe pulse primarily acts as a convolution of the vibrational population induced by the pump pulse, so that a reduction of the probe pulse duration enables to resolve better the transient features of the anti-Stokes SERS signal (note that reducing the probe pulse duration degrades the spectral resolution of the SERS peaks, so that a balance must be found. This issue is further discussed in Section S3). In conclusion, Fig. S4 shows that conclusions equivalent to those drawn in Section III. C of the main text also holds in the more general case of Fermi resonances involving 3 vibrations with a non-zero detuning of the resonance.

### C. Signatures of IVR under continuous-wave infrared pumping

In this section of the SI, we perform a similar analysis of the individual IVR pathways as in Section S2 A, but here we consider continuous-wave IR pumping and continuous-wave probing with visible light. We first focus on a Fermi resonance with  $\omega_A = 2\omega_B$ , and provide more details about the model used to obtain the results presented in Section III.D of the main text. We then analyze and discuss the more general case of a Fermi resonance with  $\omega_A \approx \omega_B + \omega_C$ .

#### 1. Fermi resonance with $\omega_A = 2\omega_B$

In the section, we discuss in more details the analysis made in Section III.D of the main text. We consider a total Hamiltonian  $\hat{\mathcal{H}}_{\text{tot}}(t) = \hat{\mathcal{H}}_{\text{VIB,A}} + \hat{\mathcal{H}}_{\text{VIB,B}} + \hat{\mathcal{H}}_{\text{F}} + \hat{\mathcal{H}}_{\text{IR,A}}(t) + \hat{\mathcal{H}}_{\text{VIS}}(t)$ , where  $\hat{\mathcal{H}}_{\text{VIB},i}$  describes the energy of the vibration  $i$  (see Eq. (1) of the main text),  $\hat{\mathcal{H}}_{\text{F}}$  accounts for the coupling of vibrations A and B by a Fermi resonance (see Eq. (9) of the main text),  $\hat{\mathcal{H}}_{\text{IR,A}}(t)$  describes the coupling between vibration A and an IR cavity illuminated by cw IR laser light (see Eq. (6) of the main text), and  $\hat{\mathcal{H}}_{\text{VIS}}(t)$  describes the coupling of the two vibrations with an optical cavity that is illuminated by cw visible laser light (see Eq. (2) of the main text). In this configuration, the IR illumination resonantly pumps vibration A while the visible light induces anti-Stokes SERS processes that enable to probe the population of the two vibrations. Accordingly, and following a similar approach and the same definitions as in Sections S1 A, S1 B and S1 C, the total Hamiltonian can be cast into the form:

$$\begin{aligned} \hat{\mathcal{H}}_{\text{tot}}(t) = & \hbar\omega_A \hat{b}_A^\dagger \hat{b}_A + \hbar\omega_B \hat{b}_B^\dagger \hat{b}_B + \hbar g_{\text{F}} (\hat{b}_A (\hat{b}_B^\dagger)^2 + \hat{b}_A^\dagger \hat{b}_B^2) + \hbar(\omega_{\text{VIS}}^{\text{cav}} - \omega_{\text{VIS}}) \hat{a}_{\text{VIS}}^\dagger \hat{a}_{\text{VIS}} + \hbar(\omega_{\text{IR}}^{\text{cav}} - \omega_{\text{IR}}) \hat{a}_{\text{IR}}^\dagger \hat{a}_{\text{IR}} \\ & - \hbar g_{\text{VIS,A}} |\alpha_{\text{VIS}}| (\hat{a}_{\text{VIS}}^\dagger + \hat{a}_{\text{VIS}}) (\hat{b}_A^\dagger + \hat{b}_A) - \hbar g_{\text{VIS,A}} \hat{a}_{\text{VIS}}^\dagger \hat{a}_{\text{VIS}} (\hat{b}_A^\dagger + \hat{b}_A) \\ & - \hbar g_{\text{VIS,B}} |\alpha_{\text{VIS}}| (\hat{a}_{\text{VIS}}^\dagger + \hat{a}_{\text{VIS}}) (\hat{b}_B^\dagger + \hat{b}_B) - \hbar g_{\text{VIS,B}} \hat{a}_{\text{VIS}}^\dagger \hat{a}_{\text{VIS}} (\hat{b}_B^\dagger + \hat{b}_B) \\ & - \hbar g_{\text{IR,A}} |\alpha_{\text{IR}}| (\hat{b}_A e^{i\omega_{\text{IR}} t} + \hat{b}_A^\dagger e^{-i\omega_{\text{IR}} t}) - \hbar g_{\text{IR,A}} (\hat{a}_{\text{IR}}^\dagger \hat{b}_A e^{i\omega_{\text{IR}} t} + \hat{a}_{\text{IR}} \hat{b}_A^\dagger e^{-i\omega_{\text{IR}} t}), \end{aligned} \quad (\text{S60})$$

where  $\alpha_{\text{IR}} = \Omega_{\text{IR}}^{\text{cw}} / [i(\omega_{\text{IR}}^{\text{cav}} - \omega_{\text{IR}}) + \kappa_{\text{IR}}/2]$ . We note that, differently to Eq. (S22), here the change in rotating frame  $e^{i\omega_{\text{IR}} t} \hat{b}_i \rightarrow \hat{b}_i$  is not applied because, in the case considered in this section, this transformation does not result in a time-independent Hamiltonian. We also note that coupling of vibration B to the IR cavity is neglected as they are strongly detuned for the parameters considered in this work ( $\omega_B \ll \omega_{\text{IR}}^{\text{cav}} - \kappa_{\text{IR}}$ , see Sec. III A of the main text). According to Eqs. (S4) and (S20), the master equation of the {molecule - IR cavity - optical cavity} system is thus:

$$\partial_t \hat{\rho} = \frac{i}{\hbar} [\hat{\rho}(t), \hat{\mathcal{H}}_{\text{tot}}(t)] + \frac{\kappa_{\text{VIS}}}{2} \mathcal{D}_{\hat{a}_{\text{VIS}}}[\hat{\rho}] + \frac{\kappa_{\text{IR}}}{2} (n_{\text{cav}}^{\text{th}} + 1) \mathcal{D}_{\hat{a}_{\text{IR}}}[\hat{\rho}] + \frac{\kappa_{\text{IR}}}{2} n_{\text{cav}}^{\text{th}} \mathcal{D}_{\hat{a}_{\text{IR}}^\dagger}[\hat{\rho}] + \sum_{i=A,B} \frac{\gamma_i(1 + n_i^{\text{th}})}{2} \mathcal{D}_{\hat{b}_i}[\hat{\rho}] + \sum_{i=A,B} \frac{\gamma_i n_i^{\text{th}}}{2} \mathcal{D}_{\hat{b}_i^\dagger}[\hat{\rho}]. \quad (\text{S61})$$

A first option to obtain the populations of the states and vibrational spectra for the configuration studied in this section is to fully implement Eq. (S61) with a numerical solver. The black lines in Fig. S5 show calculations of the states populations with this procedure, for the parameters given in Section III. A and III. D of the main text. The simulations are performed in QuTiP by evolving Eq. (S61) until a steady-state is reached for the quantities studied. Hilbert spaces with 3 number states for the vibrational operators and 2 for the cavity operators have been considered. A second option to obtain state populations and vibrational spectra is to introduce the linearization and adiabatic elimination of both the visible cavity and IR cavity operators. Applying the procedures of Sections S1 A and S1 B on Eq. (S61) yields the simplified master equation for the reduced density matrix  $\hat{\rho}_{\text{VIB}}$  of the system composed of

vibration A and B:

$$\begin{aligned} \partial_t \hat{\rho}_{\text{vib}} = & \frac{i}{\hbar} \left[ \hat{\rho}_{\text{vib}}, \hbar(\omega_A - \omega_{\text{IR}}) \hat{b}_A^\dagger \hat{b}_A + \hbar(\omega_B - \omega_{\text{IR}}/2) \hat{b}_B^\dagger \hat{b}_B + \hbar g_F (\hat{b}_A (\hat{b}_B^\dagger)^2 + \hat{b}_A^\dagger \hat{b}_B^2) - \hbar g_{\text{IR},A} |\alpha_{\text{IR}} (\hat{b}_A + \hat{b}_A^\dagger) \right] \\ & + \sum_{i=A,B} \frac{1}{2} [\gamma_i (1 + n_i^{\text{th}}) + \Gamma_i^-] \mathcal{D}_{\hat{b}_i} [\hat{\rho}_{\text{vib}}] + \sum_{i=A,B} \frac{1}{2} [\gamma_i n_i^{\text{th}} + \Gamma_i^+] \mathcal{D}_{\hat{b}_i^\dagger} [\hat{\rho}_{\text{vib}}], \end{aligned} \quad (\text{S62})$$

where the system Hamiltonian is now time-independent. The blue dashed lines in Fig. S5 show calculations with QuTiP of the states populations using this procedure and 3 number states for the vibrational operators. Lastly, state populations can be calculated semi-analytically using approximated equations for the vibrational populations and coherences derived from Eq. (S62). The corresponding closed set of equations takes the form:

$$\frac{d\langle \hat{b}_A \rangle}{dt} = -[i(\omega_A - \omega_{\text{IR}}) + \frac{\gamma_A + \Gamma_A^- - \Gamma_A^+}{2}] \langle \hat{b}_A \rangle + i g_{\text{IR},A} \alpha_{\text{IR}} - i g_F \langle \hat{b}_B^2 \rangle, \quad (\text{S63})$$

$$\frac{d\langle \hat{b}_B^2 \rangle}{dt} = -[i(2\omega_B - \omega_{\text{IR}}) + \gamma_B + \Gamma_B^- - \Gamma_B^+] \langle \hat{b}_B^2 \rangle - 2i g_F \langle \hat{b}_A \rangle (1 + 2n_B), \quad (\text{S64})$$

$$\frac{dn_A}{dt} = -(\gamma_A + \Gamma_A^-) n_A + \Gamma_A^+ (n_A + 1) + \gamma_A n_A^{\text{th}} + 2g_F \text{Im}[\langle \hat{b}_B^2 \hat{b}_A^\dagger \rangle] + 2g_{\text{IR},A} \text{Im}[\alpha_{\text{IR}}^* \langle \hat{b}_A \rangle], \quad (\text{S65})$$

$$\frac{dn_B}{dt} = -(\gamma_B + \Gamma_B^-) n_B + \Gamma_B^+ (n_B + 1) + \gamma_B n_B^{\text{th}} - 4g_F \text{Im}[\langle \hat{b}_B^2 \hat{b}_A^\dagger \rangle], \quad (\text{S66})$$

$$\frac{d\langle \hat{b}_B^2 \hat{b}_A^\dagger \rangle}{dt} = -\left[ -i(\omega_A - 2\omega_B) + \frac{(\gamma_A + \Gamma_A^- - \Gamma_A^+ + 2\gamma_B + 2\Gamma_B^- - 2\Gamma_B^+)}{2} \right] \langle \hat{b}_B^2 \hat{b}_A^\dagger \rangle - i g_F [4n_B n_A + 2n_A - (\langle \hat{n}_B^2 \rangle - n_B)], \quad (\text{S67})$$

$$\frac{d\langle \hat{n}_B^2 \rangle - n_B}{dt} = -2(\langle \hat{n}_B^2 \rangle - n_B) \times (\gamma_B + \Gamma_B^- - \Gamma_B^+) + 4n_B (\gamma_B n_B^{\text{th}} + \Gamma_B^+) - 4g_F \text{Im}[\langle \hat{b}_B^2 \hat{b}_A^\dagger \rangle] (1 + 2n_B), \quad (\text{S68})$$

where the approximations  $\langle \hat{n}_B \hat{n}_A \rangle \rightarrow n_A n_B$ ,  $\langle \hat{n}_B \hat{b}_B^2 \hat{b}_A^\dagger \rangle \rightarrow n_B \langle \hat{b}_B^2 \hat{b}_A^\dagger \rangle$  and  $\langle \hat{n}_B \hat{b}_A \rangle \rightarrow n_B \langle \hat{b}_A \rangle$  have been introduced. As in Section S2 A, the population of the subset of states  $\{|1, 0\rangle, |0, 2\rangle, |0, 1\rangle\}$  can be extracted from Eqs. (S63-S68) using  $n_{|1,0\rangle} \approx n_A$ ,  $n_{|0,2\rangle} \approx \langle \hat{n}_B^2 \rangle - n_B$  and  $n_{|0,1\rangle} \approx n_B - n_{|0,2\rangle}$ . The green dotted lines in Fig. S5 show the results calculated using this procedure. Fig. S5 clearly shows that the agreement between the three models is very good in all panels and in the whole range of IR intensities considered.

Finally, we note that it has proven difficult to obtain vibrational spectra using the full master equation Eq. S61. Indeed, due to the combination of the complexity and time-dependence of the Hamiltonian (S60), we calculated explicitly the two-times correlation in Eq. (S11)), which produces numerical artifacts in the anti-Stokes part of the final spectrum (i.e in the Fourier transform of the time correlation). Instead, the spectra in Fig. 5 (b) of the main text are calculated using the simplified (after linearization and adiabatic elimination) equations (S62), (S12) and (S13), for which such calculations are easier. However, the very good agreement of the populations predicted by the full model (Eq. (S61)) and the model after linearization and adiabatic elimination (Eq. (S62)) supports the assumption that these approximations are also accurate for the calculation of the SERS spectra.

## 2. Fermi resonance with $\omega_A \approx \omega_B + \omega_C$

In this section, we analyze the possibility to identify IVR using cw IR pumping and cw anti-Stokes SERS probing (see Fig. S6 (a)) in the case of a Fermi resonance involving 3 different molecular vibrational modes A, B and C with a non-perfect resonance condition  $\omega_A \approx \omega_B + \omega_C$ . This analysis can be performed starting from the Hamiltonian:

$$\begin{aligned} \hat{\mathcal{H}}_{\text{tot}}(t) = & \hbar\omega_A \hat{b}_A^\dagger \hat{b}_A + \hbar\omega_B \hat{b}_B^\dagger \hat{b}_B + \hbar\omega_C \hat{b}_C^\dagger \hat{b}_C + \hbar g_F (\hat{b}_A \hat{b}_B^\dagger \hat{b}_C^\dagger + \hat{b}_A^\dagger \hat{b}_B \hat{b}_C) + \hbar(\omega_{\text{VIS}}^{\text{cav}} - \omega_{\text{VIS}}) \hat{a}_{\text{VIS}}^\dagger \hat{a}_{\text{VIS}} + \hbar(\omega_{\text{IR}}^{\text{cav}} - \omega_{\text{IR}}) \hat{a}_{\text{IR}}^\dagger \hat{a}_{\text{IR}} \\ & - \hbar g_{\text{VIS},A} |\alpha_{\text{VIS}}| (\hat{a}_{\text{VIS}}^\dagger + \hat{a}_{\text{VIS}}) (\hat{b}_A^\dagger + \hat{b}_A) - \hbar g_{\text{VIS},A} \hat{a}_{\text{VIS}}^\dagger \hat{a}_{\text{VIS}} (\hat{b}_A^\dagger + \hat{b}_A) \\ & - \hbar g_{\text{VIS},B} |\alpha_{\text{VIS}}| (\hat{a}_{\text{VIS}}^\dagger + \hat{a}_{\text{VIS}}) (\hat{b}_B^\dagger + \hat{b}_B) - \hbar g_{\text{VIS},B} \hat{a}_{\text{VIS}}^\dagger \hat{a}_{\text{VIS}} (\hat{b}_B^\dagger + \hat{b}_B) \\ & - \hbar g_{\text{VIS},C} |\alpha_{\text{VIS}}| (\hat{a}_{\text{VIS}}^\dagger + \hat{a}_{\text{VIS}}) (\hat{b}_C^\dagger + \hat{b}_C) - \hbar g_{\text{VIS},C} \hat{a}_{\text{VIS}}^\dagger \hat{a}_{\text{VIS}} (\hat{b}_C^\dagger + \hat{b}_C) \\ & - \hbar g_{\text{IR},A} |\alpha_{\text{IR}}| (\hat{b}_A e^{i\omega_{\text{IR}} t} + \hat{b}_A^\dagger e^{-i\omega_{\text{IR}} t}) - \hbar g_{\text{IR},A} (\hat{a}_{\text{IR}}^\dagger \hat{b}_A e^{i\omega_{\text{IR}} t} + \hat{a}_{\text{IR}} \hat{b}_A^\dagger e^{-i\omega_{\text{IR}} t}). \end{aligned} \quad (\text{S69})$$

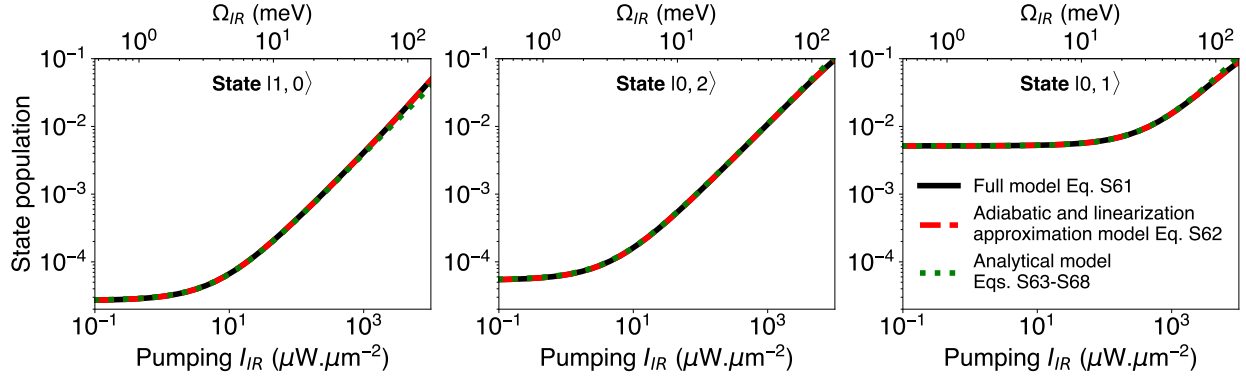

FIG. S5. Comparison of models used to analyze the importance of IVR under cw IR resonant pumping and cw anti-Stokes SERS probing. The panels show the evolution of the population of state  $|1, 0\rangle$  (left), state  $|0, 2\rangle$  (center) and state  $|0, 1\rangle$  (right) with the intensity of the IR pumping laser. Black lines show results obtained by solving the full master equation (S61). Red dashed lines are obtained by solving the master equation (S62) accounting for linearization and adiabatic elimination of the cavity degrees of freedom. The green dotted lines correspond to solutions of the set of approximated equations (S63-S68). Parameters:  $\hbar\omega_{\text{vis}} = \hbar\omega_{\text{vis},1}^{\text{cav}} = 1.96$  eV,  $\hbar\kappa_{\text{vis}} = 160$  meV,  $\hbar\Omega_{\text{vis}}[\text{meV}] = 1.13\sqrt{I_{\text{vis}}[\mu\text{W}.\mu\text{m}^{-2}]}$ ,  $\hbar\omega_{\text{ir}} = \hbar\omega_{\text{ir}}^{\text{cav}} = \hbar\omega_A$  136 meV,  $\hbar\kappa_{\text{ir}} = 12$  meV,  $\hbar\Omega_{\text{ir}}[\text{meV}] = 1.48\sqrt{I_{\text{ir}}[\mu\text{W}.\mu\text{m}^{-2}]}$ ,  $\hbar\omega_A = 136$  meV,  $\hbar\omega_B = 68$  meV,  $\hbar g_F = 1.0$  meV,  $g_{\text{ir},A} = 0.018$  meV,  $g_{\text{vis},A} = 0.021$  meV,  $g_{\text{vis},B} = 0.006$  meV,  $\gamma_A = \gamma_B = 1.2$  meV and  $T = 200$  K, Hilbert spaces with 3 number states for the vibrational operators and 2 for the cavity operators.

The corresponding master equation is then similar to Eq. (S61), provided that the sums over  $i = A, B$  are extended to vibration C. As in the previous section, the calculation of SERS spectra using the master equation is difficult due to the time-dependence of the Hamiltonian. Hence, we consider in this section linearization of the Hamiltonian and adiabatic elimination of the visible and IR cavity degrees of freedom (see Sections. S1 A, S1 B). Fig. S6 shows calculations with QuTiP (using 3 number states for the Hilbert spaces of each vibration) of (b) vibrational populations and (c) SERS spectra in this configuration. In essence, Fig. S6 (c) shows that when the IR laser is turned on with a sufficient intensity (red line), a large enhancement of the SERS peaks corresponding to vibrations B and C is observed compared to the reference case in which the laser is turned off (blue line). Such enhancement is not observed when there is no Fermi resonance between vibrations A, B and C ( $g_F = 0$ , not shown). Hence, the origin of the enhancement lies in the population transfer induced by the Fermi resonance. This enhancement of the SERS signal increases linearly with IR pumping intensity for  $I_{\text{ir}} \gtrsim 10 \mu\text{W}.\mu\text{m}^{-2}$  (as the populations scales linearly with intensity in this range, see Fig. S6 (b)). These observations directly generalize to the case of a Fermi resonance involving 3 non-perfectly resonant vibrations the conclusions reached in Section III. D of the main text. Finally, note that the temperature of the molecule considered here is  $T = 200$  K, which is higher than in the case studied in the main text. This is due to the higher IR coupling strength of the mode pumped ( $\hbar g_{\text{ir}} = 0.075$  meV here against  $\hbar g_{\text{ir}} = 0.018$  meV in the main text). This highlights that, depending on the mode pumped, high cryogenic temperatures (and possibly room temperature in some cases) could be used.

We focus next on the enhancement of the peak at frequency  $\sim \omega_A$  in Fig. S6 (c) under strong pumping (red line). On the one hand, the very narrow line at the IR laser frequency corresponds to coherent anti-Stokes SERS emission (i.e. sum-frequency generation) as analyzed in detail in Section III. D of the main text. On the other hand, Fig. S6 (c) shows that the incoherent emission by vibration A (broad peak at frequencies  $\sim \omega_A$ ) is strongly enhanced under pumping. This feature can be explained as follows. First, the coherent IR pumping induces a coherent population in state  $|1, 0, 0\rangle$ , as shown in Fig. S6 (b) by the near equality between the population of state  $|1, 0, 0\rangle$  (red line) and the coherent population  $|\langle 0, 0, 0 | \hat{\rho}_{\text{vib}} | 1, 0, 0 \rangle|^2$  (red dots) for pumping intensities  $I_{\text{ir}} \gtrsim 1 \mu\text{W}.\mu\text{m}^{-2}$ . Part of this coherent population is transferred to state  $|0, 1, 1\rangle$  by the Fermi resonance in a coherent process, as shown in Fig. S6 (b) by the near equality between the population of state  $|0, 1, 1\rangle$  (orange line) and the coherent population  $|\langle 0, 0, 0 | \hat{\rho}_{\text{vib}} | 0, 1, 1 \rangle|^2$  (orange dots) for pumping intensities  $I_{\text{ir}} \gtrsim 1 \mu\text{W}.\mu\text{m}^{-2}$ . Next, part of the excess population of state  $|0, 1, 1\rangle$  is transferred by non-radiative relaxation (at rates  $\gamma_B$  and  $\gamma_C$  respectively) to the fundamentals of vibrations B and C (states  $|0, 1, 0\rangle$  and  $|0, 0, 1\rangle$  respectively). The population in these latter states is fully incoherent ( $|\langle 0, 0, 0 | \hat{\rho}_{\text{vib}} | 0, 1, 1 \rangle|^2 = |\langle 0, 0, 0 | \hat{\rho}_{\text{vib}} | 0, 1, 1 \rangle|^2 = 0$ , not shown). A fraction of this incoherent population can then be transferred back to state  $|0, 1, 1\rangle$  by non-radiative channels (i.e. via the term  $\propto \gamma_B n_i^{\text{th}}$  in the master equation). This produces an incoherent contribution on top of the coherent population in state  $|0, 1, 1\rangle$ , which can be further transferred to state  $|1, 0, 0\rangle$  by the Fermi resonance coupling. This incoherent population is small compared to the

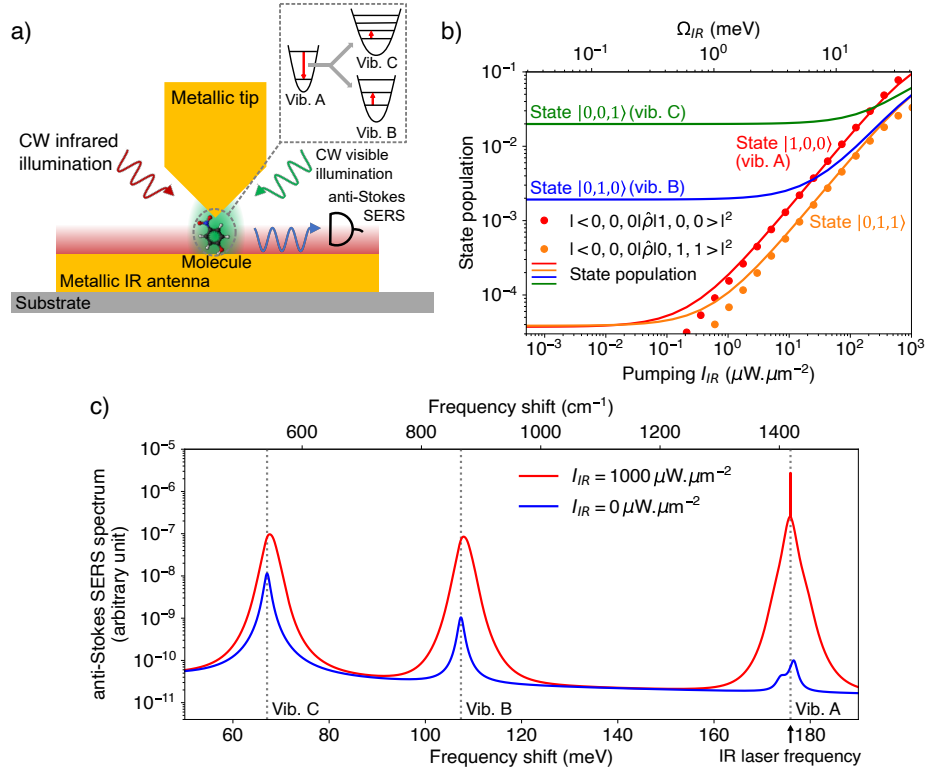

FIG. S6. *Signatures of IVR under cw IR pumping and cw anti-Stokes SERS probing for a Fermi resonance involving 3 non-perfectly resonant vibrations.* (a): sketch of the configuration under study, which consists in a single molecule in a plasmonic gap nanocavity that supports one mode at visible wavelengths (resonance at 633 nm, green shadowing on the figure, corresponding to mode 1 in Section III. A of the main text). The bottom mirror of the nanocavity is a flat metallic disk that supports a plasmonic resonance in the infrared range (mode at  $9.1 \mu m$ , or, equivalently, 136 meV, corresponding to the IR mode in Section III. A of the main text), which is responsible for an enhancement of the electric field at the position of the molecule (dark red shadowing on the figure). The IR mode is resonantly illuminated with continuous-wave IR light (dark red arrow) that resonantly pumps a single molecular vibration. The visible cavity mode is resonantly illuminated by continuous-wave visible light (green arrow) that produces an anti-Stokes SERS signal that allows monitoring the vibrational populations (blue arrow). (b): evolution of the populations of states  $|1,0,0\rangle$  (red line),  $|0,1,1\rangle$  (orange line),  $|0,1,0\rangle$  (blue line) and  $|0,0,1\rangle$  (green, lines) with the intensity of the pumping IR laser. The red dots show the quantity  $|\langle 0,0,0|\hat{\rho}|1,0,0\rangle|^2$ , i.e. the coherent population of state  $|1,0,0\rangle$  (here, it is almost equal to the coherent population  $|\langle \hat{b}_A \rangle|^2$  of vibration A). The orange dots show the quantity  $2|\langle 0,0,0|\hat{\rho}|0,1,1\rangle|^2$ , i.e. the coherent population of state  $|0,1,1\rangle$ . (c): anti-Stokes SERS spectra of the molecule for no pumping (blue line) and for cw IR pumping intensity  $I_{IR} = 1000 \mu W \cdot \mu m^{-2}$  (i.e.  $\Omega_{IR} = 46.8$  meV, red line). The dotted vertical gray lines are guides to the eye and indicate the frequencies of vibrations A, B and C. The coherent contribution to the peak (nearly vertical red lines at 172.9 meV) is plotted using a Lorentzian lineshape with very small width (0.003 meV) and normalized so that the spectral integral of the Lorentzian is equal to  $(\omega_{VIS} + \omega_A)^4 \Gamma_A^{-1} |\langle 0,0,0|\hat{\rho}|1,0,0\rangle|^2$  (see Eq. (5) of the main text). The value 0.003 meV has been chosen arbitrarily to mimic the linewidth of the excitation laser. Parameters:  $\hbar\omega_{VIS} = \hbar\omega_{VIS,1}^{cav} = 1.96$  eV,  $\hbar\kappa_{VIS} = 160$  meV,  $I_{VIS} = 100 \mu W \cdot \mu m^{-2}$  (i.e.  $\hbar\Omega_{VIS} = 11.3$  meV),  $\hbar\omega_{IR} = \hbar\omega_{IR}^{cav} = \hbar\omega_A = 172.9$  meV,  $\hbar\kappa_{IR} = 12$  meV,  $\hbar\Omega_{IR}[\text{meV}] = 1.48\sqrt{I_{IR}[\mu W \cdot \mu m^{-2}]}$ ,  $\hbar\omega_A = 172.9$  meV,  $\hbar\omega_B = 107.4$  meV,  $\hbar\omega_C = 67.1$  meV,  $\hbar g_F = 1.25$  meV,  $g_{IR,A} = 0.075$  meV,  $g_{VIS,A} = 0.024$  meV,  $g_{VIS,B} = 0.007$  meV,  $g_{VIS,C} = 0.006$  meV,  $\gamma_A = \gamma_B = \gamma_C = 1.2$  meV and  $T = 200$  K. The calculations comprise Hilbert spaces with 3 number states for the vibrational operators.

coherent populations (for state  $|0,1,1\rangle$ , compare orange points with orange line in Fig. S6 (b)); for state  $|1,0,0\rangle$ , compare red points with red line; the incoherent population corresponds to the difference between the line and the dots). Nevertheless, this incoherent population is larger than the thermal population, and results under strong pumping in a clear enhancement of the broad peak at frequency shifts  $\sim \omega_A$  in Fig. S6 (c). Hence, this feature is intimately linked to IVR in the present model, but note that we have observed a similar behavior in the absence of IVR by including pure dephasing of the coherent vibrational populations (not shown).

To finish, as in the previous sections, we compare the vibrational populations obtained in various levels of approximations. In the present case, the closed set of equations that needs to be solved to obtain the energy states population

is:

$$\frac{d\langle\hat{b}_A\rangle}{dt} = -[i(\omega_A - \omega_{\text{IR}}) + \frac{\gamma_A + \Gamma_A^- - \Gamma_A^+}{2}]\langle\hat{b}_A\rangle + ig_{\text{IR},A}\alpha_{\text{IR},A} - ig_F\langle\hat{b}_B\hat{b}_C\rangle, \quad (\text{S70})$$

$$\frac{d\langle\hat{b}_B\hat{b}_C\rangle}{dt} = -[i(\omega_B + \omega_C - \omega_{\text{IR}}) + \frac{\gamma_B + \Gamma_B^- - \Gamma_B^+ + \gamma_C + \Gamma_C^- - \Gamma_C^+}{2}]\langle\hat{b}_B\hat{b}_C\rangle - ig_F\langle\hat{b}_A\rangle(1 + n_B + n_C), \quad (\text{S71})$$

$$\frac{dn_A}{dt} = -(\gamma_A + \Gamma_A^-)n_A + \Gamma_A^+(n_A + 1) + \gamma_A n_A^{th} + 2g_F\text{Im}[\langle\hat{b}_A^\dagger\hat{b}_B\hat{b}_C\rangle] + 2g_{\text{IR},A}\text{Im}[\alpha_{\text{IR},A}^*\langle\hat{b}_A\rangle], \quad (\text{S72})$$

$$\frac{dn_B}{dt} = -(\gamma_B + \Gamma_B^-)n_B + \Gamma_B^+(n_B + 1) + \gamma_B n_B^{th} - 2g_F\text{Im}[\langle\hat{b}_A^\dagger\hat{b}_B\hat{b}_C\rangle], \quad (\text{S73})$$

$$\frac{dn_C}{dt} = -(\gamma_C + \Gamma_C^-)n_C + \Gamma_C^+(n_C + 1) + \gamma_C n_C^{th} - 2g_F\text{Im}[\langle\hat{b}_A^\dagger\hat{b}_B\hat{b}_C\rangle], \quad (\text{S74})$$

$$\begin{aligned} \frac{d\langle\hat{b}_A^\dagger\hat{b}_B\hat{b}_C\rangle}{dt} = & -\left[i(\omega_B + \omega_C - \omega_A) + \frac{(\gamma_A + \Gamma_A^- - \Gamma_A^+ + \gamma_B + \Gamma_B^- - \Gamma_B^+ + \gamma_C + \Gamma_C^- - \Gamma_C^+)}{2}\right]\langle\hat{b}_A^\dagger\hat{b}_B\hat{b}_C\rangle \\ & - ig_F[n_A(1 + n_B + n_C) - \langle\hat{n}_B\hat{n}_C\rangle] - ig_{\text{IR},A}\alpha_{\text{IR},A}^*\langle\hat{b}_B\hat{b}_C\rangle \end{aligned} \quad (\text{S75})$$

$$\begin{aligned} \frac{d\langle\hat{n}_B\hat{n}_C\rangle}{dt} = & -(\gamma_B + \Gamma_B^- - \Gamma_B^+ + \gamma_C + \Gamma_C^- - \Gamma_C^+)\langle\hat{n}_B\hat{n}_C\rangle + (\gamma_B n_B^{th} + \Gamma_B^+)n_C + (\gamma_C n_C^{th} + \Gamma_C^+)n_B \\ & - 2g_F\text{Im}[\langle\hat{b}_A^\dagger\hat{b}_B\hat{b}_C\rangle](1 + n_B + n_C), \end{aligned} \quad (\text{S76})$$

where we have used the approximations  $\langle\hat{b}_A\hat{n}_B\rangle \rightarrow \langle\hat{b}_A\rangle n_B$ ,  $\langle\hat{b}_A\hat{n}_C\rangle \rightarrow \langle\hat{b}_A\rangle n_C$ ,  $\langle\hat{n}_A\hat{n}_B\rangle \rightarrow n_A n_B$ ,  $\langle\hat{n}_A\hat{n}_C\rangle \rightarrow n_A n_C$ ,  $\langle\hat{n}_B\hat{b}_A^\dagger\hat{b}_B\hat{b}_C\rangle \rightarrow \langle\hat{b}_A^\dagger\hat{b}_B\hat{b}_C\rangle n_B$  and  $\langle\hat{n}_C\hat{b}_A^\dagger\hat{b}_B\hat{b}_C\rangle \rightarrow \langle\hat{b}_A^\dagger\hat{b}_B\hat{b}_C\rangle n_C$ . Fig. S7 shows a comparison of the evolution with IR pumping intensity of the vibrational populations for the model based on the full master equation (continuous blue lines, corresponding to Eq. (S69)), the model based on linearization and adiabatic elimination of the cavities degrees of freedom (red dashed lines) and of the semi-analytical model (green dotted lines). The agreement found between the three models is excellent.

### S3. DISCUSSION: ADDITIONAL CONSIDERATIONS

In this section, we complement the discussion in Section IV. of the main text regarding the experimental feasibility of IVR detection using SERS platforms.

- *Influence of probe pulse duration:* In Section III. C of the main text and Section S2 B 2 of the SI, we have discussed the possibility to characterize a Fermi resonance under pulsed Stokes SERS pumping and pulsed anti-Stokes SERS probing. In this configuration, the finite temporal width of the pulsed light used for probing introduces a spectral broadening of the anti-Stokes SERS signal. In particular, the Gaussian probe pulse considered in Section III. C of the main text has an amplitude  $\Omega_{\text{VIS}}^{\text{probe}}(t - t^{\text{probe}}) = \Omega_{\text{VIS}}^{\text{probe,max}} e^{-2 \ln(2) \times [(t - t^{\text{probe}})/\Delta\tau^{\text{probe}}]^2}$  and a central frequency  $\omega_{\text{VIS},1}^{\text{CAV}}$ , which gives the non-monochromatic Fourier transform  $\Omega_{\text{VIS}}^{\text{probe}}(\omega, t^{\text{probe}}) \propto e^{-(\omega - \omega_{\text{VIS},1}^{\text{CAV}})^2 \times (\Delta\tau^{\text{probe}})^2 / 8 \ln(2)}$ . The corresponding intensity spectrum ( $|\Omega_{\text{VIS}}^{\text{probe}}(\omega)|^2$ ) has a width at half maximum  $4 \ln(2) / \Delta\tau^{\text{probe}}$  (FWHM), corresponding to 4.6 meV ( $37 \text{ cm}^{-1}$ ) for a probe pulse with  $\Delta\tau^{\text{probe}} = 400$  fs. The value is of the same order of magnitude as the vibrational linewidth  $\gamma_i$  and is smaller than the typical energy spacing between vibrational modes in Raman spectra. Hence, the spectral broadening for  $\Delta\tau^{\text{probe}} \gtrsim 400$  fs should not hinder accurate measurements of the anti-Stokes SERS signal. Importantly, we have shown that such pulse durations provide sufficient time resolution to capture the temporal signatures of IVR.

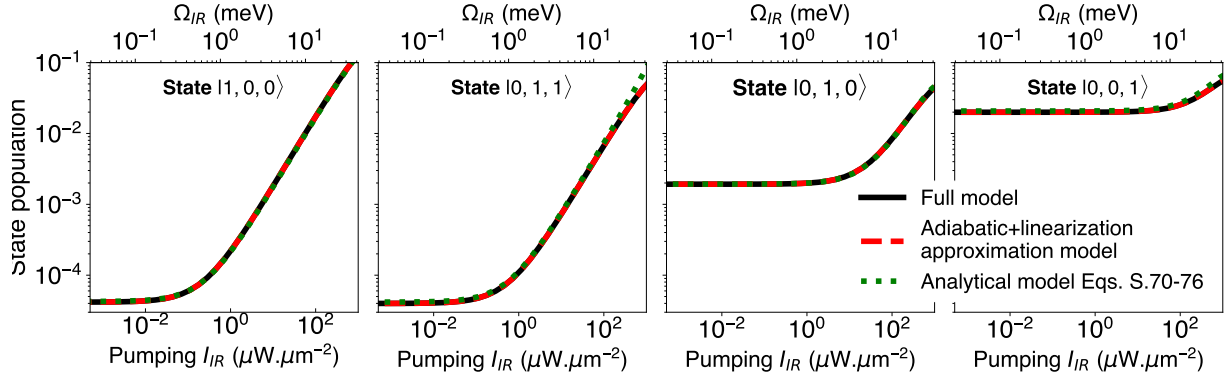

FIG. S7. Comparison of models used to analyze the importance of IVR under cw IR resonant pumping and cw anti-Stokes SERS probing for a Fermi resonance involving 3 non-perfectly resonant vibrations. The different panels show the evolution of the population of state  $|1, 0, 0\rangle$  (left), state  $|0, 1, 1\rangle$  (center left), state  $|0, 1, 0\rangle$  (center right) and  $|0, 0, 1\rangle$  (right) with IR pumping intensity. Black lines show results obtained by solving the full master equation, red dashed lines are obtained by solving the master equation after linearization and adiabatic elimination of the cavity degrees of freedom, and the green dotted lines correspond to solutions of the set of approximated Eqs. (S70-S76). Parameters:  $\hbar\omega_{\text{VIS}} = \hbar\omega_{\text{VIS},1}^{\text{cav}} = 1.96$  eV,  $\hbar\kappa_{\text{VIS}} = 160$  meV,  $I_{\text{VIS}} = 100 \mu\text{W}.\mu\text{m}^{-2}$  (i.e.  $\hbar\Omega_{\text{VIS}} = 11.3$  meV),  $\hbar\omega_{\text{IR}} = \hbar\omega_{\text{IR}}^{\text{cav}} = \hbar\omega_A = 172.9$  meV,  $\hbar\kappa_{\text{IR}} = 12$  meV,  $\hbar\Omega_{\text{IR}}[\text{meV}] = 1.48\sqrt{I_{\text{IR}}[\mu\text{W}.\mu\text{m}^{-2}]}$ ,  $\hbar\omega_A = 172.9$  meV,  $\hbar\omega_B = 107.4$  meV,  $\hbar\omega_C = 67.1$  meV,  $\hbar g_F = 1.25$  meV,  $g_{\text{IR},A} = 0.075$  meV,  $g_{\text{VIS},A} = 0.024$  meV,  $g_{\text{VIS},B} = 0.007$  meV,  $g_{\text{VIS},C} = 0.006$  meV,  $\gamma_A = \gamma_B = \gamma_C = 1.2$  meV and  $T = 200$  K. The calculations comprise Hilbert spaces with 2 number states for all the operators.

- Selectivity of vibrational mode pumping by Stokes SERS:** In this work, we have considered the case of two or three vibrational modes in a molecule, but realistic molecules can contain tens of modes. Therefore, it is essential to control the pumped vibrational mode to accurately characterize a given IVR pathway. For the technique based on cw IR laser pumping, this constraint is satisfied as the linewidth of a cw IR laser is narrow compared to a vibrational linewidth and to the energy difference between vibrations, so that a single vibration can be pumped resonantly in the molecule. For the technique based on pulsed SERS pumping, a challenge arises because SERS induces a broadband excitation process. Nevertheless, we note that most molecules only feature a few strong Raman lines (i.e. with large optomechanical coupling strengths  $g_{\text{VIS}}$ ). The NBT molecule studied in this work represents a relevant example (see e.g. a SERS spectrum of NBT in [S30]). In this case, the vibrational modes that are strongly excited are well separated in energy, such that the Fermi resonances responsible for their relaxation likely involve distinct low-energy vibrational modes. Additionally, several options are available to provide selective modal excitation. First, according to Eq. (4) of the main text and Eq. (S8) of the SI, Stokes SERS pumping of a vibration  $i$  is maximized when  $\omega_{\text{VIS}} - \omega_{\text{VIS}}^{\text{cav}} = \omega_i$ , so that selective pumping of a given vibration can be partly controlled by adjusting the laser and/or cavity frequency. For the parameter  $\kappa_{\text{VIS}} = 160$  meV considered in this work, the selectivity of pumping would remain relatively small, but can be enough to strongly pump a high energy vibrational mode A while modestly pumping the other low-energy modes (as desired for the configuration studied in Section III. B and C of the main text). The advent of hybrid plasmonic-dielectric cavities [S31, S32] also offers an alternative route to achieve highly sideband-selective Raman vibrational enhancements. Lastly, selective vibrational pumping may be achieved by stimulated Raman scattering, that is by using an additional laser detuned by  $-\omega_i$  from the primary pumping laser to stimulate Stokes Raman scattering in the vibrational mode  $i$ .
- Influence of collective effects due to the presence of multiple molecules:** We have studied the case of a single molecule, but we consider here the case of several identical molecules in a SERS platform. Recent studies have shown that the anti-Stokes SERS signal from an assembly of  $N$  molecules scales with  $N^2$  when the vibrations are pumped out-of-equilibrium by the Stokes SERS processes [S9, S33]. A similar statement holds when the vibrations are pumped out-of-equilibrium by an IR resonant laser [S19]. This is due to a collective effect arising from the coupling of all the molecules to the same plasmonic (visible or IR) modes. However, according to the theory introduced in this work, the presence of many molecules will strengthen the total signal but the sensitivity of the IVR detection will not be otherwise affected by these collective effects. First, we note that IVR is a redistribution effect occurring in each individual molecules, and not a collective phenomenon, because it involves the potential energy surface of a single molecule. Hence, the efficiency of population transfer between vibrations only depends on the out-of-equilibrium populations reached in each individual molecule under

pumping. At the same time, the collective effects mentioned above only affect the anti-Stokes SERS signal, not the individual vibrational populations. Accordingly, the collective effects do not enhance the out-of-equilibrium populations induced in each molecule under pumping and thus the population transferred by IVR to the other vibrations. Finally, we speculate that collective effects might appear when the molecules are in physical contact, leading to a collective potential energy surface, but including such effect in our model is left for future studies.

- *IVR of low energy vibrations:* In this work, we have discussed methods to characterize IVR in molecules, focusing on vibrational modes with relatively high energy (several tens of meV). For these modes, Fermi resonances (i.e. IVR) are expected to be the main relaxation pathways [S29]. We note that for lower energy vibrational modes, other relaxation channels involving, e.g., coupling to metal, solvent or intermolecular phonon modes (i.e. extra-molecular relaxation) may play a major role [S34, S35]. For example, metallic phonon modes lie roughly in the range 0-25 meV (0-200  $\text{cm}^{-1}$ ) [S36]. Similar numbers are found for intermolecular coupling effect between molecular vibrations in self-assembled monolayers [S37]. Hence, our formalism would need to be extended for the study of IVR pathways involving vibrational modes with typical energy  $\lesssim 30$  meV ( $\lesssim 250 \text{ cm}^{-1}$ ).
- *Further considerations on molecular anharmonicities:* In this work, we have focused on molecular anharmonicities that couple together several molecular vibrations. On the other hand, for a given vibrational mode, anharmonicities can also lead to significant deviations from the equal state energy spacing found in the harmonic approximation (due to terms  $U_{i,i,i}^{(3)}\hat{q}_i^3$ ,  $U_{i,i,i,i}^{(4)}\hat{q}_i^4$  and higher orders contributions in the molecular Hamiltonian, see Eq. (8) of the main text and [S38]). However, we expect that this effect have negligible or relatively weak effect on our analysis of IVR. Indeed, these anharmonicities have no effect on  $g_F$  and do not prevent the resonance condition between the high-energy mode and the overtone (or combination) of the low-energy mode(s) from being satisfied, which are the two main factors before the Fermi resonance coupling strength.

## S4. DFT CALCULATIONS OF THE VIBRATIONAL PROPERTIES

### A. Details of the DFT calculations

In this section we describe the details of the DFT calculations performed to compute the vibrational properties (vibrational frequencies, IR dipole moments, Raman tensors and anharmonic couplings) of the molecule studied. We choose to use DFT, rather than alternative methods such as, e.g., the second-order Møller-Plesset perturbation theory (MP2) implemented in Ref. [S29], because DFT is a less computationally demanding approach, and thus enables us to address IVR in larger molecular systems, such as NBT attached to gold nanostructures. Additionally, it has been recently highlighted that MP2 fails to accurately describe potential energy surfaces of planar aromatic molecules, as it is the case with NBT [S39]. In particular, we perform DFT calculations for the bare NBT molecule, NBT with one gold atom attached (AuNBT), and NBT attached to a tetrahedral cluster formed by 19 gold atoms ( $\text{Au}_{19}\text{NBT}$ ). We obtain the structure of the cluster by removing one gold atoms from the 20-atoms gold structure used in Ref. [S40]. In the case of NBT and AuNBT, we first optimize the structure within DFT using the exchange-correlation functional B3LYP [S41], which shows good performance for computing fundamental frequencies and anharmonic effects [S39, S42], and the basis set 6-31G(d,p) [S43], for the atoms of hydrogen, carbons, nitrogen, oxygen and sulfur. We use the basis set LANL2DZ [S44] for the atoms of gold of the cluster. We then use these minimum energy structures to compute the vibrational properties (vibrational frequencies, IR dipole moments, Raman tensors and anharmonic couplings) at the same level of theory (B3LYP/6-31G(d,p)/LANL2DZ). All the vibrational frequencies have been found to be positive, which confirms that the molecular structure corresponds to energy minima of the potential energy surface (see the optimized structures in Figure S8). In the case of  $\text{Au}_{19}\text{NBT}$ , we use the same basis set (6-31G(d,p)/LANL2DZ) and exchange-correlation functional (B3LYP) than those used for computing the vibrational properties for AuNBT, but we add the semiempirical correction D3 of Grimme in conjunction with the damping function of Becke and Johnson (BJ), [S45, S46], which accounts for the non-covalent interactions between the molecule and the cluster. Additionally, we freeze the position of the gold atoms of the cluster during the optimization and computation of the vibrational properties, so that we can separate the vibrational modes localized to the molecule from those delocalized between the molecule and the cluster. The molecular structure obtained corresponds to a minimum of the potential energy surfaces as no imaginary frequencies have been obtained. We computed anharmonic effects within deperturbed second-order vibrational perturbation theory (DVPT2) approach [S47] for NBT, AuNBT and  $\text{Au}_{19}\text{NBT}$ . We use the code Gaussian 16 Rev. B. 01 [S48] to carry out all the DFT calculations. We use the software VMD version 1.9.4 to generate the images of the atomistic models in Figure S8. [S49].

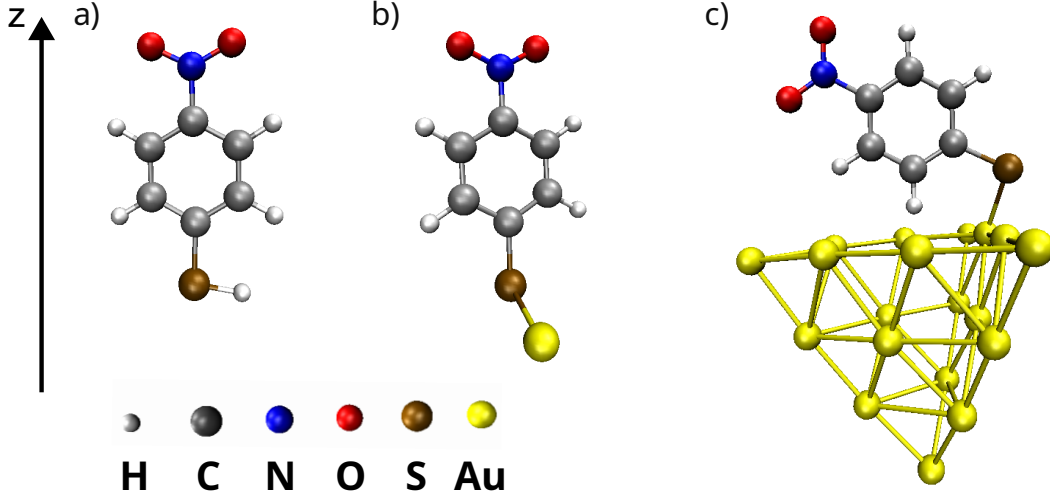

FIG. S8. Atomistic model of the structures of the NBT molecule attached to gold atoms. Optimized structure obtained within DFT for the (a) bare NBT molecule, (b) AuNBT and (c) Au<sub>19</sub>NBT. These structures were used to compute the vibrational properties studied in this work. The axis  $z$  stands for the direction normal to the metallic surface.

### B. Fermi resonances studied in this work

The Fermi resonance studied in the main text is based on the interaction between the carbon-sulfur stretching mode (mode A) and a low-energy vibration (mode B) that is characterized by antiphase relative motions of the nitro group (NO<sub>2</sub>) and the phenyl ring (see Figure S9). In particular, this interaction results in a coupling between the fundamental energy state of vibration A and the overtone of vibration B, which is called a Fermi resonance. As shown in Table S1, DFT calculations with 19 atoms of gold yield the Fermi resonance coupling strength  $\hbar g_F = 13.48 \text{ cm}^{-1} = 1.67 \text{ meV}$ , and the vibrational frequencies  $\hbar\omega_A = 1099.94 \text{ cm}^{-1} = 136.4 \text{ meV}$  and  $\hbar\omega_B = 541.17 \text{ cm}^{-1} = 67.1 \text{ meV}$ . In Section S1 C, the effect of the detuning between the fundamental of mode A and the overtone of mode B, here  $\hbar(\omega_A - 2\omega_B) = 17.60 \text{ cm}^{-1}$ , is shown to reduce effectively the strength of the Fermi resonance. For simplicity, in the main text, we consider a perfectly resonant Fermi resonance with  $\omega_A = 2\omega_B = 136 \text{ meV}$ , and take into account the effective reduction of  $g_F$  using Eq. (S35), which yields  $\hbar g_F = 8.01 \text{ cm}^{-1} = 1.0 \text{ meV}$  (using  $\hbar\gamma_A = \hbar\gamma_B = 1.2 \text{ meV}$ , see Section III.A of the main text).

In this Supplementary Information (Sections S2 A 2, S2 B 2 and S2 C 2), we also consider a Fermi resonance of the type  $\omega_A \approx \omega_B + \omega_C$ . This Fermi resonance results from the interaction between the symmetric stretching mode of the nitrogen-oxygen bonds of the nitro group (NO<sub>2</sub>; mode A), the symmetric bending mode of the nitro group (mode B) and the low-energy vibration at  $541.17 \text{ cm}^{-1}$  (here mode C. Note that this is also mode B in the previous Fermi resonance  $\omega_A = 2\omega_B$ ). As shown in Table S2, DFT calculations with 19 atoms of gold yield the Fermi resonance coupling strength  $\hbar g_F = 10.10 \text{ cm}^{-1} = 1.25 \text{ meV}$ , and the vibrational frequencies  $\hbar\omega_A = 1394.53 \text{ cm}^{-1} = 172.9 \text{ meV}$ ,  $\hbar\omega_B = 866.15 \text{ cm}^{-1} = 107.4 \text{ meV}$  and  $\hbar\omega_C = 541.17 \text{ cm}^{-1} = 67.1 \text{ meV}$ . In this case, we directly implement in our calculations these bare values.

### C. Effect of the gold atoms on the Fermi couplings for NBT

We evaluate next the impact of the gold atoms covalently bonded to the NBT molecule on the Fermi resonances analyzed in this work. In Tables S1 and S2, we show the frequencies and couplings for the bare molecule of NBT, and the molecule with one (AuNBT) and nineteen (Au<sub>19</sub>NBT) gold atoms attached. In both tables, we find that the presence of the gold atoms has a little effect on the frequencies for the selected vibrational modes. For example, in the case of the Fermi resonance  $\omega_A = 2\omega_B$  (Table S1), the maximum shifts for modes A and B are  $21.8 \text{ cm}^{-1}$  and  $7.9 \text{ cm}^{-1}$ , respectively. Nevertheless, these little differences can have a significant influence on the detuning between the fundamental of mode A and the overtone of mode B or the combination of modes B and C, which modulates the effective strength of the Fermi resonance (see Eq. (S35)). In the two tables, we also find that the coupling  $g_F$  is quenched by the introduction of one gold atom (and even completely suppressed for the Fermi resonance of Table S2),

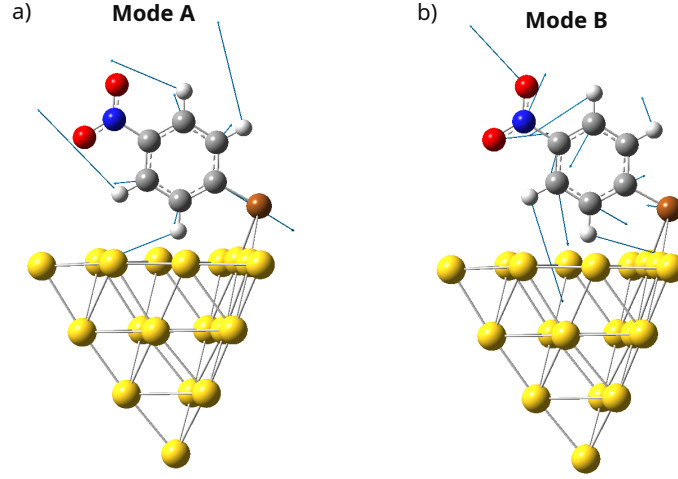

FIG. S9. *Vibrational motifs for the modes participating in the selected Fermi resonance for  $\text{Au}_{19}\text{NBT}$ .* (a): mode A at frequency  $1099.94 \text{ cm}^{-1}$ . (b): mode B at frequency  $541.17 \text{ cm}^{-1}$ . The overtone of mode B couples to mode A. The thin arrows point towards the direction of the atomic displacements. The spheres colored white, gray, blue, red, brown and yellow represent the atoms of hydrogen, carbon, nitrogen, oxygen, sulfur and gold, respectively.

and is then mostly restored when the 19-atom gold cluster is attached to the molecule. In summary, these changes do not affect the main conclusions of our work, as they modify the exact quantitative values but not the qualitative behavior. However, we emphasize that their effect can be significant and thus require careful analysis for quantitative theoretical studies of IVR in molecules embedded in plasmonic structures.

|                            | $\hbar\omega_A$ | $\hbar\omega_B$ | $\hbar \omega_A - 2\omega_B $ | $\hbar g_F$ |
|----------------------------|-----------------|-----------------|-------------------------------|-------------|
| NBT                        | 1116.67         | 536.30          | 44.07                         | 17.42       |
| AuNBT                      | 1094.89         | 533.30          | 28.29                         | 5.72        |
| $\text{Au}_{19}\text{NBT}$ | 1099.94         | 541.17          | 17.60                         | 13.48       |

TABLE S1. *Effect of the gold atoms on a Fermi resonance  $\omega_A = 2\omega_B$  of NBT.* Second and third columns: vibrational frequencies computed with DFT for the modes A (second column) and B (third column) participating in the Fermi resonance studied in the main text and in Figs. S1, S5 of the SI. Fourth column: difference between the frequency of mode A, and the frequency of the first overtone (second harmonic;  $2\omega_B$ ) of mode B. Fifth column: coupling strength ( $g_F$ ), in absolute value, of the Fermi resonances. All the quantities in the table are in  $\text{cm}^{-1}$ .

|                            | $\hbar\omega_A$ | $\hbar\omega_B$ | $\hbar\omega_C$ | $\hbar \omega_A - \omega_B - \omega_C $ | $\hbar g_F$ |
|----------------------------|-----------------|-----------------|-----------------|-----------------------------------------|-------------|
| NBT                        | 1393.62         | 864.72          | 536.30          | 7.4                                     | 11.96       |
| AuNBT                      | 1398.22         | 865.53          | 533.30          | 0.61                                    | 0.00        |
| $\text{Au}_{19}\text{NBT}$ | 1394.53         | 866.15          | 541.17          | 12.88                                   | 10.10       |

TABLE S2. *Effect of the gold atoms on a Fermi resonance  $\omega_A \approx \omega_B + \omega_C$  of NBT.* Second, third and fourth columns: vibrational frequencies computed with DFT for the modes A (second column), B (third column) and C (fourth column) participating in the Fermi resonance studied in Figs. S2,S3,S4,S6 and S7 of the SI. Fifth column: difference between the frequency of mode A, and the frequencies of modes B and C. Sixth column: coupling strength ( $g_F$ ), in absolute value, of the Fermi resonances. All the quantities in the table are in  $\text{cm}^{-1}$ .

- 
- [S1] P. Roelli, C. Galland, N. Piro, and T. J. Kippenberg, Molecular cavity optomechanics as a theory of plasmon-enhanced Raman scattering, *Nature nanotechnology* **11**, 164 (2016).  
[S2] M. K. Schmidt, R. Esteban, A. González-Tudela, G. Giedke, and J. Aizpurua, Quantum mechanical description of Raman scattering from molecules in plasmonic cavities, *ACS nano* **10**, 6291 (2016).

- [S3] R. Esteban, J. J. Baumberg, and J. Aizpurua, Molecular optomechanics approach to surface-enhanced Raman scattering, *Accounts of Chemical Research* **55**, 1889 (2022).
- [S4] P. Roelli, H. Hu, E. Verhagen, S. Reich, and C. Galland, Nanocavities for molecular optomechanics: Their fundamental description and applications, *ACS photonics* **11**, 4486 (2024).
- [S5] R. Esteban, J. Aizpurua, and G. W. Bryant, Strong coupling of single emitters interacting with phononic infrared antennae, *New Journal of Physics* **16**, 013052 (2014).
- [S6] M. K. Schmidt, R. Esteban, F. Benz, J. J. Baumberg, and J. Aizpurua, Linking classical and molecular optomechanics descriptions of SERS, *Faraday Discussions* **205**, 31 (2017).
- [S7] E. Le Ru and P. Etchegoin, *Principles of Surface-Enhanced Raman Spectroscopy: and related plasmonic effects* (Elsevier, 2008).
- [S8] J. J. Baumberg, J. Aizpurua, M. H. Mikkelsen, and D. R. Smith, Extreme nanophotonics from ultrathin metallic gaps, *Nature materials* **18**, 668 (2019).
- [S9] Y. Zhang, J. Aizpurua, and R. Esteban, Optomechanical collective effects in surface-enhanced Raman scattering from many molecules, *ACS Photonics* **7**, 1676 (2020).
- [S10] H.-P. Breuer and F. Petruccione, *The theory of open quantum systems* (OUP Oxford, 2002).
- [S11] I. Wilson-Rae, N. Nooshi, W. Zwerger, and T. J. Kippenberg, Theory of ground state cooling of a mechanical oscillator using dynamical backaction, *Physical review letters* **99**, 093901 (2007).
- [S12] P. Degenfeld-Schonburg, M. Abdi, M. J. Hartmann, and C. Navarrete-Benlloch, Degenerate optomechanical parametric oscillators: Cooling in the vicinity of a critical point, *Physical Review A* **93**, 023819 (2016).
- [S13] M. Kamandar Dezfouli and S. Hughes, Quantum optics model of surface-enhanced raman spectroscopy for arbitrarily shaped plasmonic resonators, *ACS Photonics* **4**, 1245 (2017).
- [S14] M. Aspelmeier, T. J. Kippenberg, and F. Marquardt, Cavity optomechanics, *Reviews of Modern Physics* **86**, 1391 (2014).
- [S15] L. A. Jakob, W. M. Deacon, Y. Zhang, B. de Nijs, E. Pavlenko, S. Hu, C. Carnegie, T. Neuman, R. Esteban, J. Aizpurua, *et al.*, Giant optomechanical spring effect in plasmonic nano-and picocavities probed by surface-enhanced Raman scattering, *Nature Communications* **14**, 3291 (2023).
- [S16] A. Kavokin, J. J. Baumberg, G. Malpuech, and F. P. Laussy, *Microcavities* (Oxford university press, 2017).
- [S17] H. J. Carmichael, *Statistical methods in quantum optics 1: master equations and Fokker-Planck equations* (Springer Science & Business Media, 2013).
- [S18] C. Cohen-Tannoudji, J. Dupont-Roc, and G. Grynberg, *Atom-photon interactions: basic processes and applications* (John Wiley & Sons, 2024).
- [S19] P. Roelli, D. Martin-Cano, T. J. Kippenberg, and C. Galland, Molecular platform for frequency upconversion at the single-photon level, *Physical Review X* **10**, 031057 (2020).
- [S20] P. W. Atkins and R. S. Friedman, *Molecular quantum mechanics* (Oxford university press, 2011).
- [S21] W. Chen, P. Roelli, H. Hu, S. Verlekar, S. P. Amirtharaj, A. I. Barreda, T. J. Kippenberg, M. Kovylyna, E. Verhagen, A. Martínez, *et al.*, Continuous-wave frequency upconversion with a molecular optomechanical nanocavity, *Science* **374**, 1264 (2021).
- [S22] A. Xomalis, X. Zheng, R. Chikkaraddy, Z. Koczor-Benda, E. Miele, E. Rosta, G. A. Vandenbosch, A. Martínez, and J. J. Baumberg, Detecting mid-infrared light by molecular frequency upconversion in dual-wavelength nanoantennas, *Science* **374**, 1268 (2021).
- [S23] P. Törmä and W. L. Barnes, Strong coupling between surface plasmon polaritons and emitters: a review, *Reports on Progress in Physics* **78**, 013901 (2014).
- [S24] T. Neuman and J. Aizpurua, Origin of the asymmetric light emission from molecular exciton-polaritons, *Optica* **5**, 1247 (2018).
- [S25] More rigorously, if the system is in the strong coupling regime, the Lindblad terms needs to be derived in the eigenbasis (S36). This introduces a modification of the master equation in Eq. (S29), which becomes in principle more relevant as the coupling strength increases [S50]. However, the system studied in this work is at the limit between weak and strong coupling, and we expect this more rigorous approach to modify the results only weakly even for large coupling strengths ( $2\sqrt{2}g_F \gg \gamma_A + \gamma_B$ ), so that we let the exploration of this effect for future studies.
- [S26] J. R. Johansson, P. D. Nation, and F. Nori, Qutip: An open-source python framework for the dynamics of open quantum systems, *Computer physics communications* **183**, 1760 (2012).
- [S27] J. Johansson, P. Nation, and F. Nori, Qutip 2: A python framework for the dynamics of open quantum systems, *Computer Physics Communications* **184**, 1234 (2013).
- [S28] N. Lambert, E. Giguère, P. Menczel, B. Li, P. Hopf, G. Suárez, M. Gali, J. Lishman, R. Gadhvi, R. Agarwal, *et al.*, Qutip 5: The quantum toolbox in python, *arXiv preprint arXiv:2412.04705* (2024).
- [S29] H. Poudel, P. H. Shaon, and D. M. Leitner, Vibrational energy flow in molecules attached to plasmonic nanoparticles, *The Journal of Physical Chemistry C* (2024).
- [S30] E. L. Keller and R. R. Frontiera, Ultrafast nanoscale raman thermometry proves heating is not a primary mechanism for plasmon-driven photocatalysis, *ACS nano* **12**, 5848 (2018).
- [S31] I. Shlesinger, I. M. Palstra, and A. F. Koenderink, Integrated sideband-resolved sers with a dimer on a nanobeam hybrid, *Physical Review Letters* **130**, 016901 (2023).
- [S32] I. Shlesinger, J. Vandersmissen, E. Oksenberg, E. Verhagen, and A. F. Koenderink, Hybrid cavity-antenna architecture for strong and tunable sideband-selective molecular Raman scattering enhancement, *Science Advances* **9**, eadj4637 (2023).
- [S33] L. A. Jakob, A. Juan-Delgado, N. S. Mueller, S. Hu, R. Arul, R. A. Boto, R. Esteban, J. Aizpurua, and J. J. Baumberg, Optomechanical pumping of collective molecular vibrations in plasmonic nanocavities, *ACS nano* (2025).

- [S34] V. Kenkre, A. Tokmakoff, and M. Fayer, Theory of vibrational relaxation of polyatomic molecules in liquids, *The Journal of chemical physics* **101**, 10618 (1994).
- [S35] A. Nitzan, *Chemical dynamics in condensed phases: relaxation, transfer, and reactions in condensed molecular systems* (Oxford university press, 2024).
- [S36] A. Dal Corso, A. Pasquarello, and A. Baldereschi, Density-functional perturbation theory for lattice dynamics with ultrasoft pseudopotentials, *Physical Review B* **56**, R11369 (1997).
- [S37] A. Boehmke Amoruso, R. A. Boto, E. Elliot, B. de Nijs, R. Esteban, T. Földes, F. Aguilar-Galindo, E. Rosta, J. Aizpurua, and J. J. Baumberg, Uncovering low-frequency vibrations in surface-enhanced raman of organic molecules, *Nature Communications* **15**, 6733 (2024).
- [S38] D. A. McQuarrie, *Quantum chemistry* (University Science Books, 2008).
- [S39] N. Palanisamy and S. Banik, Exploring the accuracy of density functionals for anharmonic vibrations of polycyclic aromatic hydrocarbons, *The Journal of Physical Chemistry A* **129**, 7794 (2025).
- [S40] R. A. Boto, R. Esteban, B. Candelas, and J. Aizpurua, Theoretical procedure for precise evaluation of chemical enhancement in molecular surface-enhanced raman scattering, *The Journal of Physical Chemistry C* **128**, 18293 (2024).
- [S41] A. D. Becke, Density-functional thermochemistry. iii. the role of exact exchange, *The Journal of chemical physics* **98**, 5648 (1993).
- [S42] J. Neugebauer and B. A. Hess, Fundamental vibrational frequencies of small polyatomic molecules from density-functional calculations and vibrational perturbation theory, *The Journal of chemical physics* **118**, 7215 (2003).
- [S43] G. Petersson and M. A. Al-Laham, A complete basis set model chemistry. ii. open-shell systems and the total energies of the first-row atoms, *The Journal of chemical physics* **94**, 6081 (1991).
- [S44] P. J. Hay and W. R. Wadt, Ab initio effective core potentials for molecular calculations. potentials for k to au including the outermost core orbitals, *The Journal of chemical physics* **82**, 299 (1985).
- [S45] S. Grimme, J. Antony, S. Ehrlich, and H. Krieg, A consistent and accurate ab initio parametrization of density functional dispersion correction (dft-d) for the 94 elements h-pu, *The Journal of chemical physics* **132** (2010).
- [S46] S. Grimme, S. Ehrlich, and L. Goerigk, Effect of the damping function in dispersion corrected density functional theory, *Journal of computational chemistry* **32**, 1456 (2011).
- [S47] V. Barone, Anharmonic vibrational properties by a fully automated second-order perturbative approach, *The Journal of chemical physics* **122**, 014108 (2005).
- [S48] M. J. Frisch, G. W. Trucks, H. B. Schlegel, G. E. Scuseria, M. A. Robb, J. R. Cheeseman, G. Scalmani, V. Barone, G. A. Petersson, H. Nakatsuji, X. Li, M. Caricato, A. V. Marenich, J. Bloino, B. G. Janesko, R. Gomperts, B. Mennucci, H. P. Hratchian, J. V. Ortiz, A. F. Izmaylov, J. L. Sonnenberg, D. Williams-Young, F. Ding, F. Lipparini, F. Egidi, J. Goings, B. Peng, A. Petrone, T. Henderson, D. Ranasinghe, V. G. Zakrzewski, J. Gao, N. Rega, G. Zheng, W. Liang, M. Hada, M. Ehara, K. Toyota, R. Fukuda, J. Hasegawa, M. Ishida, T. Nakajima, Y. Honda, O. Kitao, H. Nakai, T. Vreven, K. Throssell, J. A. Montgomery, Jr., J. E. Peralta, F. Ogliaro, M. J. Bearpark, J. J. Heyd, E. N. Brothers, K. N. Kudin, V. N. Staroverov, T. A. Keith, R. Kobayashi, J. Normand, K. Raghavachari, A. P. Rendell, J. C. Burant, S. S. Iyengar, J. Tomasi, M. Cossi, J. M. Millam, M. Klene, C. Adamo, R. Cammi, J. W. Ochterski, R. L. Martin, K. Morokuma, O. Farkas, J. B. Foresman, and D. J. Fox, *Gaussian 16 Revision B.01* (2016), gaussian Inc. Wallingford CT.
- [S49] W. Humphrey, A. Dalke, and K. Schulten, VMD – Visual Molecular Dynamics, *Journal of Molecular Graphics* **14**, 33 (1996).
- [S50] T. Neuman, R. Esteban, G. Giedke, M. K. Schmidt, and J. Aizpurua, Quantum description of surface-enhanced resonant raman scattering within a hybrid-optomechanical model, *Physical Review A* **100**, 043422 (2019).
